# Supplementary material for: Covariance-engaged Classification of Sets via Linear Programming
Source: arXiv:2006.14831 source file (2020-06-26)
Supplement: Supplementary file 1 [file CLIPS_supp.pdf]

# Covariance-engaged Classification of Sets via Linear Programmin

Zhao Ren, Sungkyu Jung and Xingye Qiao

*University of Pittsburgh, Seoul National University, Binghamton University*

**Supplementary Material**

## S1. Theoretical Properties under Time Series Structures

We consider the performance of CLIPS classifier when observations within each set are allowed to follow various time series structures, and extend the results obtained in Theorems 3, 4, 5 and 6 in these dependent settings.

We follow the assumption in Section 2 that both the $N$ sets $\{(\mathcal{X}_i, \mathcal{Y}_i)\}_{i=1}^N$ and the new set $(\mathcal{X}^\dagger, \mathcal{Y}^\dagger)$ are generated in the same way as $(\mathcal{X}, \mathcal{Y})$ independently. In this section, the generating process of $(\mathcal{X}, \mathcal{Y})$ is generalized to allow both short-range and long-range dependent time series. Specifically, while we still assume $\mathcal{Y}$ and $M$ are independent with class probabilities $\pi_k$ $(k = 1, 2)$ and distribution $p_M$ respectively, here we assume that conditioned on $M = m$ and $\mathcal{Y} = y$, observations $X_1, X_2, \ldots, X_m$ in the set $\mathcal{X}$ follow a vector linear process,

$$X_i = \mu_y + \sum_{t=0}^{\infty} A_{yt}\xi_{i-t}, \tag{S1.1}$$

where $A_{yt}$ are $p \times p$ dimensional coefficient matrices in class $\mathcal{Y} = y$ and $\xi_t = (\xi_{t1}, \ldots, \xi_{tp})^T$ with $(\xi_{tj})_{t\in\mathbb{Z}, j=1,\ldots,p}$ being i.i.d. standard normal variables. Note that the covariance matrices of individual observation from two classes are $\Sigma_y := \Sigma_{y0} = \sum_{t=0}^{\infty} A_{yt}A_{yt}^T$ for $y = 1, 2$. In general, the auto-covariance matrices at lag $k$ of all observations within each set, that is

$\mathrm{Cov}(X_i, X_{i+k}) := \Sigma_{yk} = \sum_{t=0}^{\infty} A_{yt} A_{y(t+k)}^T$ for $y = 1, 2$. The above vector linear process is flexible since the coefficient matrices $A_{yt}$ can capture both spatial and temporal dependences. One important example is the vector auto-regression (VAR) model. It has been widely used in many fields, including functional Magnetic Resonance Imagine (fMRI) and microarray data (Dinov et al., 2005; Posekany et al., 2011).

To characterize the dependence relationship of the time series, we impose conditions on the coefficient matrices. Set $A_{yt} = (a_{yt,ij})_{1\le i,j\le p}$. Then we assume the Gaussian linear process satisfies the following decay condition on $A_{yt}$ for both classes $y = 1, 2$, and all $t \ge 0$,

$$\max_{1\le i\le p} (\sum_{j=1}^{p} a_{yt,ij}^2)^{1/2} \le C_{TS}(1+t)^{-\nu}, \tag{S1.2}$$

where $C_{TS} > 0$ is some constant and $\nu > 1/2$ reflects the decay rate. The requirement $\nu > 1/2$ is needed to guarantee that the covariance matrix $\Sigma_y = \sum_{t=0}^{\infty} A_t A_t^T$ is finite. In particular, in the time series literature, when $\nu > 1$, the corresponding linear process is said to have a short-range dependence (SRD) because rows of the the corresponding auto-covariance matrices $\Sigma_{yk}$ are absolutely summable, which yields relatively weak dependence among all observations within each set. When $1/2 < \nu < 1$, the corresponding auto-covariance matrices may not be absolutely summable and thus the linear process is said have a long-range dependence (LRD). See, for example Beran (2017); Wu et al. (2010) for more details.

We investigate generalization errors for the CLIPS classifier $\tilde{\phi}(\mathcal{X}^\dagger)$ in (3.12) under the vector linear process model for both short-rang and long-range dependence. It is worthwhile pointing out that $\phi_B$ in (2.2) is no longer the Bayes decision rule due to the time series structure. In contrast, the full Bayes decision rule for model (S1.1) requires the knowledge

of all coefficient matrices $A_{yt}$ for $t \in \mathbb{Z}, y = 1, 2$. However, in high-dimensional situations, it is difficult to estimate all coefficient matrices $A_{yt}$ accurately if not impossible at all. With the decay condition (S1.2), it is still reasonable to apply some simplified quadratic classier such as $\phi_B(\mathcal{X}^\dagger)$ in (2.2) to predict $\mathcal{Y}^\dagger$ as if all observations in the test set $\mathcal{X}^\dagger$ are independent. Indeed, under the independence case in which $A_{yt} = 0$ for all $t \geq 1$, $\phi_B(\mathcal{X}^\dagger)$ is the oracle of our CLIPS classifier $\tilde{\phi}(\mathcal{X}^\dagger)$. With the general time series structure (S1.1), we need to define the oracle of our CLIPS first.

$$\tilde{\phi}(\mathcal{X}^\dagger) = 2 - \mathbb{1}\left\{\frac{\log(\hat{\pi}_1/\hat{\pi}_2)}{m} + \tilde{\beta}_0 + \tilde{\beta}^T \bar{x} + \bar{x}^T \tilde{\nabla} \bar{x}/2 + \operatorname{tr}(\tilde{\nabla} S)/2 > 0\right\}.$$

Recall that the key estimation in our CLIPS classifier displayed above include quadratic term $\tilde{\nabla}$, linear coefficient $\tilde{\beta}$ and an intercept coefficient $\tilde{\beta}_0$. While the estimations $\tilde{\nabla}$ in (3.8) and $\tilde{\beta}$ in (3.9) are proposed to estimate their counterparts in our CLIPS classifier $\nabla = \Sigma_2^{-1} - \Sigma_1^{-1}$ and $\beta = \beta_1 - \beta_2$ where $\beta_y = \Sigma_y^{-1}\mu_y$ respectively, the constant coefficient estimator $\tilde{\beta}_0$ in (3.10) is obtained via a logistic regression model. Therefore, the oracle $\beta_{0,TS}$ of $\tilde{\beta}_0$ in the current setting is defined as the minimizer of the following population loss function, that is,

$$\beta_{0,TS} = \underset{\theta_0 \in \mathbb{R}}{\operatorname{argmin}} \ \mathbb{E}\ell(\theta_0 \mid \{(\mathcal{X}_i, \mathcal{Y}_i)\}_{i=1}^N, \beta, \nabla), \tag{S1.3}$$

where $\ell(\theta_0 \mid \{(\mathcal{X}_i, \mathcal{Y}_i)\}_{i=1}^N, \beta, \nabla)$ is defined in (3.11). We point out the interpretation of $\ell(\cdot)$ is no longer the negative log-likelihood function and thus $\beta_{0,TS}$ is not always equal to the quantity $\beta_0 = \{-\log(|\Sigma_1|/|\Sigma_2|) - \mu_1^T \Sigma_1^{-1} \mu_1 + \mu_2^T \Sigma_2^{-1} \mu_2\}/2$ defined in (2.2). However, the oracle classifier $\phi_{B,TS}$ of CLIPS defined below is always no worse (i.e., has the same or smaller generalization error) than $\phi_B$ in (2.2) due to its definition (S1.3). Again, for the independence case, we have $\phi_{B,TS} = \phi_B$.

$$\phi_{B,TS}(\mathcal{X}^\dagger) = 2 - \mathbb{1}\left\{\frac{\log(\pi_1/\pi_2)}{m} + \beta_{0,TS} + \beta^T \bar{x} + \bar{x}^T \nabla \bar{x}/2 + \operatorname{tr}(\nabla S)/2 > 0\right\}. \tag{S1.4}$$

From now on, we denote by $R_{B,TS}$ the oracle risk although the subscript $B$ no longer implies the Bayes decision rule.

We first extend Theorem 3 and establish the statistical properties of the thresholded CLIME difference estimator $\tilde{\nabla}$ defined in (3.8). Again, we assume that the true quadratic parameter $\nabla = \Sigma_2^{-1} - \Sigma_1^{-1} \in \mathcal{FM}_0(s_q)$ has sparsity no more than $s_q$ defined in (4.13).

**Theorem 1.** *Consider the vector linear process defined in (S1.1) that satisfies the decay condition (S1.2). Suppose Conditions 1-3 hold. Moreover, assume* $\nabla \in \mathcal{FM}_0(s_q)$, $\|\Sigma_k^{-1}\|_{\ell_1} \leq C_{\ell 1}$ *with some constant* $C_{\ell 1} > 0$ *for* $k = 1, 2$ *and* $\log p \leq c_0 N$ *with some sufficiently small constant* $c_0 > 0$. *Then for any fixed* $L > 0$, *with probability at least* $1 - O(p^{-L})$, *we have that*

$$\begin{aligned} \|\tilde{\nabla} - \nabla\|_\infty &\leq 2\lambda'_{1,N}, \\ \|\tilde{\nabla} - \nabla\|_F &\leq 2\sqrt{s_q}\lambda'_{1,N}, \\ \|\tilde{\nabla} - \nabla\|_1 &\leq 2s_q\lambda'_{1,N}, \end{aligned}$$

*as long as* $\lambda'_{1,N} \geq 8C_{\ell 1}\lambda_{1,N}$ *in (3.8) and*

$$\lambda_{1,N} \geq \begin{cases} CC_{\ell 1}\sqrt{\frac{\log p}{Nm_0}} & \text{if } \nu > 3/4 \\ CC_{\ell 1}\sqrt{\frac{\log p}{Nm_0^{4\nu-2}}} & \text{if } 1/2 < \nu < 3/4 \end{cases},$$

*where* $C$ *depends on* $L, C_e, C_\pi, C_{TS}$ *and* $c_m$. *Moreover, we have* $\mathrm{pr}(\mathrm{supp}(\tilde{\nabla}) \subset \mathrm{supp}(\nabla)) = 1 - O(p^{-L})$.

**Remark 1.** The choice of tuning parameter $\lambda_{1,N}$ and the rates of convergence on the boundary case $\nu = 3/4$ can also be dealt. In particular, we require $\lambda_{1,N} \geq CC_{\ell 1}\sqrt{\frac{\log p \log m_0}{Nm_0}}$ if $\nu = 3/4$. See the proof of Theorem 1 for further details.

The results in Theorem 1 critically depend on the estimation accuracy of the sample covariance matrix under the supnorm in various time series dependence structures within each

set. Such technical results are detailed in Lemma 6 in Appendix, where the corresponding analysis requires an application of Hanson-Wright inequality. In particular, if $\nu > 3/4$, then the rates of convergence for estimating $\nabla$ are the same as those under the independence assumption. If $n < 3/4$, that is, the vector linear process has a long-range dependence, then the rates can be affected and reduced correspondingly.

We turn to the statistical properties of the linear coefficient estimator $\tilde{\beta}$ defined in (3.9) under time series structure. The following theorem is an extension of Theorem 4, in which we assume that $\beta = \beta_1 - \beta_2$ belongs to the $s_l$-sparse ball defined in (4.14).

**Theorem 2.** *Consider the vector linear process defined in (S1.1) that satisfies the decay condition (S1.2). Suppose Conditions 1-3 hold. Moreover, assume that* $\beta \in \mathcal{F}_0(s_l)$, $\log p \leq c_0 N$, $\|\beta_k\|_1 \leq C_\beta$ *and* $\|\mu_k\| \leq C_\mu$ *with some constants* $C_\beta, C_\mu > 0$ *for* $k = 1, 2$ *and some sufficiently small constant* $c_0 > 0$. *Then for any fixed* $L > 0$, *with probability at least* $1 - O(p^{-L})$, *we have that*

$$\begin{aligned} \|\tilde{\beta} - \beta\|_1 &\leq C'' C_{\ell 1} s_l \lambda_{2,N}, \\ \|\tilde{\beta} - \beta\| &\leq C'' C_{\ell 1} \sqrt{s_l} \lambda_{2,N}, \end{aligned}$$

*as long as the tuning parameter* $\lambda_{2,N}$ *in (3.9) satisfies*

$$\lambda_{2,N} \geq \begin{cases} C' \sqrt{\frac{\log p}{N m_0}} & \text{if } \nu > 1 \\ C' \sqrt{\frac{\log p}{N m_0^{2\nu - 1}}} & \text{if } 1/2 < \nu < 1 \end{cases},$$

*where* $\max\{\|\Sigma_1^{-1}\|_{\ell_1}, \|\Sigma_2^{-1}\|_{\ell_1}\} \leq C_{\ell 1}$ *and* $C'', C'$ *depend on* $L, C_e, c_m, C_\pi, C_\beta, C_{TS}$ *and* $C_\mu$.

**Remark 2.** The choice of tuning parameter $\lambda_{2,N}$ and the rates of convergence on the boundary case $\nu = 1$ can also be dealt. In particular, we require $\lambda_{2,N} \geq C' \sqrt{\frac{\log p \log^2 m_0}{N m_0}}$ if $\nu = 1$. See the proof of Theorem 2 for further details.

At a hight level, the estimation accuracy of linear coefficients are determined by both estimation accuracy of the sample mean and that of the sample covariance matrix under the supnorm. While under the short-range dependence structure both rates of convergence are equal to $\sqrt{(\log p/(Nm_0))}$, the rate of convergence of sample mean dominates that of sample covariance matrix when there is a long-range dependence among multiple observations within each set.

Next, we derive the rate of convergence for estimating the oracle constant coefficient $\beta_{0,TS}$ defined in (S1.3) under the general time series structure. The accuracy of our estimator $\tilde{\beta}_0$ critically depends on the accuracy for estimating $\beta$ and $\nabla$. Theorem 3 extends Theorem 5 from the independent case to the general time series structure. We need one mild condition, the population strong convexity of the loss function $\ell(\beta_{0,TS} \mid \{(\mathcal{X}_i, \mathcal{Y}_i)\}_{i=1}^N, \beta, \nabla)$ at the oracle point $\beta_{0,TS}$.

**Condition 1.** Set $\bar{X}$ and $S$ as the sample mean and variance of the set of observations $(\mathcal{X}, \mathcal{Y})$ with set size $M$. Define $Z_i = \log(\pi_1/\pi_2)/M + \bar{X}^T\beta + \bar{X}^T\nabla\bar{X}/2 + \mathrm{tr}(\nabla S)/2$. The expectation of the variable $\frac{\exp(M(\beta_0+Z))}{(1+\exp(M(\beta_0+Z)))^2}$ is bounded below by $C_{\log} > 0$, where $C_{\log}$ is some universal constant.

**Remark 3.** Strong convexity Condition 1 coincides with Condition 4 for the independent case. Indeed, for the independent case we have $\mathrm{Var}(\mathcal{Y} \mid \mathcal{X}) = \frac{\exp(M(\beta_0+Z))}{(1+\exp(M(\beta_0+Z)))^2}$.

**Theorem 3.** *Consider the vector linear process defined in (S1.1) that satisfies the decay condition (S1.2). Suppose Conditions 1-4 and 1 hold,* $\log p \leq c_0 N$ *with some sufficiently small constant* $c_0 > 0$ *and* $\|\mu_k\| \leq C_\mu$ *with some constant* $C_\mu > 0$ *for* $k = 1, 2$*. Besides, we have some initial estimators* $\tilde{\beta}$, $\tilde{\nabla}$, $\hat{\pi}_1$ *and* $\hat{\pi}_2$ *such that* $m_0(\|\tilde{\beta} - \beta\|_1)(1 + U_\beta) + m_0(\|\tilde{\nabla} -$

*$\nabla\|_1)(1+U_\nabla)+\max_{k=1,2}|\pi_k-\hat{\pi}_k| \le C_p$ for some sufficiently small constant $C_p>0$ with probability at least $1-O(p^{-L})$. Then, with probability at least $1-O(p^{-L})$, we have*

$$\left|\tilde{\beta}_0-\beta_0\right| \le C_\delta\left((\|\tilde{\beta}-\beta\|_1)(1+U_\beta)+(\|\tilde{\nabla}-\nabla\|_1)(1+U_\nabla)+\max_{k=1,2}|\pi_k-\hat{\pi}_k|/m_0+\sqrt{\frac{\log p}{Nm_0^2}}\right),$$

*where $U_\beta$ satisfies*

$$U_\beta=\begin{cases}\sqrt{\frac{\log p}{m_0}} & \text{if } \nu>1\\ \sqrt{\frac{\log p}{m_0^{2\nu-1}}} & \text{if } 1/2<\nu<1\end{cases},$$

*$U_\nabla$ satisfies*

$$U_\nabla=\begin{cases}\frac{\log p}{m_0} & \text{if } \nu>1\\ \frac{\log p}{m_0^{2\nu-1}} & \text{if } 1/2<\nu<1\end{cases},$$

*and constant $C_\delta$ depends on $L, C_e, C_\pi, C_{\log}, C_\mu, C_{TS}, C_m, c_m$.*

**Remark 4.** The rates of convergence on the boundary case $\nu=1$ can also be dealt. In particular, we require $U_\beta=\sqrt{\frac{\log p\log^2 m_0}{m_0}}$ and $U_\nabla=\frac{\log p\log^2 m_0}{m_0}$ if $\nu=1$. See the proof of Theorem 3 for further details.

We point out that the rate of convergence for estimating $\beta_{0,TS}$ depends on the estimation accuracy of the linear coefficient through a term $\|\tilde{\beta}-\beta\|_1$ in Theorem 3 while it relies on a potentially smaller term $\|\tilde{\beta}-\beta\|_2$ in Theorem 5 under independent assumption in Section 4. This is due to a technical reason and the result cannot be improved (i.e., replacing $\|\tilde{\beta}-\beta\|_1$ by $\|\tilde{\beta}-\beta\|_2$) if we only assume the decay condition (S1.2).

Theorems 1, 2 and 3 extend Theorems 3, 4 and 5 respectively, and demonstrate the estimation accuracy for the quadratic, linear and constant coefficients in our CLIPS classifier (3.12) under the general time series structure. Finally, we establish an oracle inequality for its generalization error via providing a rate of convergence of the excess risk. Recall the

generalization error of CLIPS classifier is $\tilde{R} = \pi_1 \tilde{R}_1 + \pi_2 \tilde{R}_2$, where $\tilde{R}_k = \text{pr}(\tilde{\phi}(\mathcal{X}^\dagger) \neq k \mid \mathcal{Y}^\dagger = k)$. Again pr is the conditional probability given the training data $\{(\mathcal{X}_i, \mathcal{Y}_i)\}_{i=1}^N$ which $\tilde{\phi}(\mathcal{X}^\dagger)$ depends on. In addition, we define the generalization error of the oracle classifier $\phi_{B,TS}$ as $R_{B,TS} = \pi_1 R_{1,TS} + \pi_2 R_{2,TS}$, where $R_{k,TS} = \text{pr}(\phi_{B,TS}(\mathcal{X}^\dagger) \neq k \mid \mathcal{Y}^\dagger = k)$.

We need to introduce some notation $d_{N,TS}$ related to the oracle classifier in (S1.4), which is similar to $d_N$ defined in Section 4 for independence case. Recall the oracle classifier $\phi_{B,TS}(\mathcal{X}^\dagger)$ solely depends on the sign of the function $g_{TS}(\mathcal{X}^\dagger) = \frac{1}{m}\log(\pi_1/\pi_2) + \beta_{0,TS} + \beta^T \bar{x} + \bar{x}^T \nabla \bar{x}/2 + \text{tr}(\nabla S)/2$. We define by $F_{k,m,TS}$ the conditional cumulative distribution function of the oracle statistic $g_{TS}(\mathcal{X}^\dagger)$ given that $M^\dagger = m$ and $\mathcal{Y}^\dagger = k$, and define by $d_{N,TS}$ the upper bound of their first derivatives for all possible $m$ near 0,

$$d_{N,TS} = \max_{m \in [c_m m_0, C_m m_0],\ k=1,2} \left\{ \sup_{t \in [-\delta_0, \delta_0]} \left| F'_{k,m,TS}(t) \right| \right\},$$

where $\delta_0$ is any sufficiently small constant. The value of $d_{N,TS}$ is determined by the vector linear process (S1.1) and performance of the oracle classifier. We define the counterparts of $\Xi_N$ and its statistical order $\kappa_N$ defined in Section 4 under the general time series structure below, which critically determine the excess risk. Indeed, one can show that Theorems 1, 2 and 3 imply that with probability at least $1 - O(p^{-L})$,

$$\Xi_{N,TS} := (1 + U_\beta)\|\tilde{\beta} - \beta\|_1 + (1 + U_\nabla)\|\tilde{\nabla} - \nabla\|_1 + \max_{k=1,2} \frac{|\hat{\pi}_k - \pi_k|}{m_0} + \left|\tilde{\beta}_0 - \beta_{0,TS}\right| = O(\kappa_{N,TS}),$$

where $\kappa_{N,TS} := (1 + U_\nabla) s_q \lambda'_{1,N} + (1 + U_\beta) C_{\ell 1} s_l \lambda_{2,N} + \sqrt{(\log p)/(N m_0^2)}$, and the key quantities $U_\beta, U_\nabla, \lambda'_{1,N}$ and $\lambda_{2,N}$ are specified in the statement of Theorems 1, 2 and 3 for various value of $\mu$. The quantity $\kappa_{N,TS} d_{N,TS}$ is the leading rate of convergence in the oracle inequality. We need one more condition to guarantee the assumptions of Theorem 3 are satisfied with high probability, which is similar to Condition 5 for independence case.

**Condition 2.** Suppose $m_0\kappa_{N,TS} \le c_0$ and $\kappa_{N,TS}d_{N,TS} \le c_0$ with some sufficiently small constant $c_0 > 0$.

Theorem 4 below reveals the oracle property of CLIPS classifier under the general time series structure.

**Theorem 4.** *Suppose that the assumptions of Theorems 1 and 2 hold and that Conditions 1–2 also hold. Then with probability at least $1 - O(p^{-L})$, we have the oracle inequality*

$$\tilde{R} \le R_{B,TS} + C_g(\kappa_{N,TS}d_{N,TS} + p^{-L}),$$

*where constant $C_g$ depends on $L, C_e, C_\pi, C_{\log}, C_\beta, C_m, c_m, C_{TS}$ and $C_\mu$ only.*

## S2. Proofs of Main Results

### Proof of Theorem 1

*Proof.* We only prove that $R_{B1} \to 0$ and the proof of $R_{B2} \to 0$ is similar. In addition note that

$$\begin{aligned} R_{Bk} &= \mathrm{pr}(\phi_B(\mathcal{X}^\dagger) \neq k \mid \mathcal{Y}^\dagger = k) \\ &= \sum_{m=c_m m_0}^{C_m m_0} \mathrm{pr}(\phi_B(\mathcal{X}^\dagger) \neq k \mid \mathcal{Y}^\dagger = k, M^\dagger = m) \cdot p_M(m) \\ : &= \sum_{m=c_m m_0}^{C_m m_0} R_{Bk,m} \cdot p_M(m), \end{aligned}$$

where the last equality is due to independence of $\mathcal{Y}^\dagger$ and $M^\dagger$, and Condition 2. Hence it is sufficient for us to focus on any fixed $m \in [c_m m_0, C_m m_0]$.

Given that the set is from Class 1, we have $X_i^\dagger \sim N(\mu_1, \Sigma_1), i = 1, \ldots, m$. The Bayes decision rule classifies the set to Class 2, i.e., $\phi_B(\mathcal{X}^\dagger) = 2$ in (2.2) if $g(X_1^\dagger, \ldots, X_m^\dagger) < 0$,

which is equivalent to

$$\sum_{i=1}^{m}\left(X_i^\dagger-\mu_1\right)^T\nabla\left(X_i^\dagger-\mu_1\right)-2m\delta^T\Sigma_2^{-1}(\bar{X}-\mu_1)+m\delta^T\Sigma_2^{-1}\delta-m\log\left(\frac{|\Sigma_1|}{|\Sigma_2|}\right)+2\log\left(\frac{\pi_1}{\pi_2}\right)<0, \tag{S2.5}$$

where $\bar{X}=\sum_{i=1}^m X_i^\dagger/m$ is the sample mean.

Define $V=\Sigma_1^{1/2}\Sigma_2^{-1}\Sigma_1^{1/2}-I$ where $I$ is the identity matrix. We set $Z_i=\Sigma_1^{-1/2}(X_i^\dagger-\mu_1)\sim N(0,I)$, $A_{m,p}=\sum_{i=1}^m Z_i^TVZ_i-2m\delta^T\Sigma_2^{-1}\Sigma_1^{1/2}\bar{Z}$ with $\bar{Z}=\sum_{i=1}^m Z_i/m$. Then the Bayes risk $R_{B1,m}$ can be written as, following from (S2.5),

$$R_{B1,m}=\mathrm{pr}\left(A_{m,p}-\mathbb{E}A_{m,p}<-\alpha\right),$$

where $\alpha=m\mathrm{tr}(V)+m\delta^T\Sigma_2^{-1}\delta-m\log\{|\Sigma_1|\,/\,|\Sigma_2|\}+2\log\left(\pi_1/\pi_2\right)$ since $\mathbb{E}A_{m,p}=m\mathrm{tr}(V)$. The strategy to bound $R_{B1,m}$ is to show that $|A_{m,p}-\mathbb{E}A_{m,p}|$ concentrates on $\sqrt{m}D_p$ but $\alpha>0$ diverges at a faster rate of $mD_p^2$.

We first give an upper bound of the magnitude of $A_{m,p}-\mathbb{E}A_{m,p}$. Write the eigen-decomposition of $V$ as $U\Lambda U^T$ and the diagonal matrix $\Lambda=\mathrm{diag}(\lambda_j)$ with $\lambda_1\geq\lambda_2\geq\ldots\geq\lambda_p$. Moreover, set $\tilde{Z}_i=U^TZ_i\sim N(0,I)$ with $\tilde{Z}_{i,j}$ its $j$th entry. Note that

$$A_{m,p}-\mathbb{E}A_{m,p}=\sum_{i=1}^{m}\sum_{j=1}^{p}\lambda_j(\tilde{Z}_{i,j}^2-1)-2m\delta^T\Sigma_2^{-1}\Sigma_1^{1/2}\bar{Z}.$$

The tail probability of normal distribution implies

$$\mathrm{pr}(|2m\delta^T\Sigma_2^{-1}\Sigma_1^{1/2}\bar{Z}|>t)\leq 2\exp\left\{-\frac{1}{2}\left(\frac{t}{2\sqrt{m}\|\delta^T\Sigma_2^{-1}\Sigma_1^{1/2}\|}\right)^2\right\}\leq 2\exp\left(-\frac{C_e^{-3}t^2}{8m\|\delta\|^2}\right), \tag{S2.6}$$

where the last inequality is due to Condition 1. Since $\tilde{Z}_{i,j}^2-1$ is sub-exponential, Bernstein's inequality (e.g. Vershynin, 2012, Proposition 5.16) implies that there exists some universal

constant $c_1 > 0$ such that

$$\mathrm{pr}(|\sum_{i=1}^{m}\sum_{j=1}^{p}\lambda_j(\tilde{Z}_{i,j}^2-1)|>t)\leq 2\exp\left(-c_1\min(\frac{t^2}{m\|\Lambda\|_F^2},\frac{t}{\max\{|\lambda_1|,|\lambda_p|\}})\right). \quad \text{(S2.7)}$$

Now we focus on the lower bound of $\alpha$. First of all, notice that $m\delta^T\Sigma_2^{-1}\delta \geq mC_e^{-1}\|\delta\|^2$ by Condition 1. Moreover, there exists some constant $c_2 > 0$ depending on $C_e$ only such that

$$\begin{aligned} m\mathrm{tr}(V)-m\log\{|\Sigma_1|/|\Sigma_2|\} &= m\left(\mathrm{tr}(V)-\log|I+V|\right) \\ &= m\sum_{j=1}^{p}(\lambda_j-\log(1+\lambda_j))\geq c_2 m\|\Lambda\|_F^2 \quad \text{(S2.8)} \end{aligned}$$

where the last inequality follows from that $\lambda_j+1\in[C_e^{-2},C_e^2]$ according to Condition 1. Note that $\|\Lambda\|_F=\|V\|_F=\|\Sigma_1^{1/2}\nabla\Sigma_1^{1/2}\|_F$ and $C_e^{-1}\leq\|V\|_F/\|\nabla\|_F\leq C_e$ according to Condition 1. Therefore by combining the above two results we conclude $\alpha\geq c_3mD_p^2+2\log(\pi_1/\pi_2)$ with $c_3=\min(c_2C_e^{-2},C_e^{-1})>0$.

Note that by Conditions 1 and 3, $\lambda_1$ in equation (S2.7) and $2\log(\pi_1/\pi_2)$ in the expression of $\alpha$ are bounded. When $mD_p^2$ is large enough, we can pick $t=cmD_p^2$ for small enough $c>0$ in equations (S2.6) and (S2.7) such that $A_{m,p}-\mathbb{E}A_{m,p}>-\alpha$ with probability at least $1-4\exp\left(-c'mD_p^2\right)$. Therefore we complete our proof by seeing that for each fixed $m$, $R_{B1,m}\leq 4\exp\left(-c'mD_p^2\right)$ for some small constant $c'>0$, together with the fact $m\in[c_mm_0,C_mm_0]$ from Condition 2. □

## Proof of Proposition 1

*Proof.* Note that instead of $m$ observations with i.i.d. $N(\mu_k,\Sigma_k)$ from either class $k=1,2$, in the current case, we only have one representative $\bar{x}\sim N(\mu_k,\Sigma_k/m)$ with $k=1$ or 2. Therefore, the proof of upper bound, i.e., $R_{\bar{x}}\leq 4\exp\left(-c'(\|\nabla\|_F^2+m_0\|\delta\|^2)\right)$ for some small constant $c'>0$, simply follows from the proof of Theorem 1 by replacing $m_0$ and $\Sigma_k$ by 1

and $\Sigma_k/m_0$ respectively.

To show the rate on the exponent cannot be further improved in general, we need a little more efforts. Following the proof procedures for Theorem 1, it is sufficient to show the same lower bound on each $R_{\bar{x}k,m} := \mathrm{pr}(\phi_{B,\bar{x}}(\mathcal{X}^\dagger) \neq k \mid \mathcal{Y}^\dagger = k, M^\dagger = m)$ where $m \in [c_m m_0, C_m m_0]$. Given that the set is from Class 1, we have $\bar{X}^\dagger \sim N(\mu_1, \Sigma_1/m)$. $\phi_{B,\bar{x}}$ classifies the set to Class 2 if $g_{QDA}(\bar{X}^\dagger) < 0$, which is equivalent to

$$m\left(\bar{X}^\dagger - \mu_1\right)^T \nabla \left(\bar{X}^\dagger - \mu_1\right) - 2m\delta^T\Sigma_2^{-1}(\bar{X}^\dagger - \mu_1) + m\delta^T\Sigma_2^{-1}\delta - \log\left(\frac{|\Sigma_1|}{|\Sigma_2|}\right) + 2\log\left(\frac{\pi_1}{\pi_2}\right) < 0.$$

Define $V = \Sigma_1^{1/2}\Sigma_2^{-1}\Sigma_1^{1/2} - I$ where $I$ is the identity matrix. Write the eigen-decomposition of $V$ as $U\Lambda U^T$ and the diagonal matrix $\Lambda = \mathrm{diag}(\lambda_j)$ with $\lambda_1 \geq \lambda_2 \geq \ldots \geq \lambda_p$. Moreover, set $Z = \sqrt{m}U^T\Sigma_1^{-1/2}(\bar{X}^\dagger - \mu_1) \sim N(0, I)$ with $Z_j$ its $j$th entry, and $A_{m,p} = \sum_{j=1}^p \lambda_j Z_j^2 - 2\sqrt{m}\delta^T\Sigma_2^{-1}\Sigma_1^{1/2}UZ$. Then the risk $R_{\bar{x}1,m}$ can be written as $R_{\bar{x}1,m} = \mathrm{pr}\left(A_{m,p} - \mathbb{E}A_{m,p} < -\alpha\right)$, where $\alpha = \sum_{j=1}^p \lambda_j + m\delta^T\Sigma_2^{-1}\delta - \log\{|\Sigma_1| \,/\, |\Sigma_2|\} + 2\log\left(\pi_1/\pi_2\right)$ since $\mathbb{E}A_{m,p} = \sum_{j=1}^p \lambda_j$. We first upper bound the value of $\alpha$. Notice that $mC_e^{-1}\|\delta\|^2 \leq m\delta^T\Sigma_2^{-1}\delta \leq mC_e\|\delta\|^2$ by Condition 1. Moreover, a similar argument to (S2.8) also provides an upper bound, i.e., for two small constants $c_2 < c_2' < 1$, we have $c_2\|\Lambda\|_F^2 \leq \sum_{j=1}^p \lambda_j - \log\{|\Sigma_1| \,/\, |\Sigma_2|\} \leq c_2'\|\Lambda\|_F^2$. By Condition 3, $2\log(\pi_1/\pi_2)$ in the expression of $\alpha$ is bounded. Therefore, under our assumption on sufficiently large $\|\nabla\|_F^2 + m_0\|\delta\|^2$, we have that $0 < \alpha < c(\|\nabla\|_F^2 + m_0\|\delta\|^2)$ with some small $c > 0$.

We show the rate on exponent cannot be further improved by showing a lower bound for some special cases of $\mu_1, \mu_2, \Sigma_1, \Sigma_2$. Assume the support of vector $(\lambda_1, ..., \lambda_p)^T$ and the support of vector $\delta^T\Sigma_2^{-1}\Sigma_1^{1/2}U$ are disjoint (e.g., both $\Sigma_k$ are diagonal matrices with difference on the first $p/2$ diagonal entries, and only the last $p/2$ coordinates on mean difference $\delta$

are nonzero). For this scenario, the first term $T_1 := \sum_{j=1}^{p} \lambda_j Z_j^2$ and second term $T_2 := -2\sqrt{m}\delta^T \Sigma_2^{-1} \Sigma_1^{1/2} U Z$ in $A_{m,p}$ are independent. To show that the term $T_1$ is non-positive with probability away from zero, we apply Proposition 2.4 in Johnstone (2001) to obtain that $\mathrm{pr}\,(T_1 < 0) > \gamma > 0$ with some absolute constant $\gamma > 0$ by noting that the first term is a weighted Chi-square variable. By tail probability of normal distribution and the upper bound of $\alpha$, we further obtain that $\mathrm{pr}\,(T_2 < -\alpha) > \exp(c(\|\nabla\|_F^2 + m_0\|\delta\|^2))$ with some small $c > 0$. In the end, by independence, we obtain that $R_{\bar{x}1,m} = \mathrm{pr}\,(A_{m,p} - \mathbb{E}A_{m,p} < -\alpha) > \exp(c(\|\nabla\|_F^2 + m_0\|\delta\|^2))\gamma > \exp(c''(\|\nabla\|_F^2 + m_0\|\delta\|^2))$ with some small $c'' > 0$, which completes our proof. □

## Proof of Theorem 2

*Proof.* We only prove that $\hat{R}_1 \to 0$ with high probability and $\hat{R}_2 \to 0$ can be shown by symmetry. The strategy of the proof is similar to that for Theorem 1. We further focus on each fixed $m \in [c_m m_0, C_m m_0]$ since

$$\begin{aligned} \hat{R}_k &= \sum_{m=c_m m_0}^{C_m m_0} \mathrm{pr}(\hat{\phi}(\mathcal{X}^\dagger) \neq k \mid \mathcal{Y}^\dagger = k, M^\dagger = m) \cdot p_M(m) \\ : &= \sum_{m=c_m m_0}^{C_m m_0} \hat{R}_{k,m} \cdot p_M(m). \end{aligned} \tag{S2.9}$$

The quadratic set classifier classifies the set to 2, that is, $\hat{\phi}(\mathcal{X}^\dagger) = 2$ in (3.6) if

$$\sum_{i=1}^{m} \left(X_i^\dagger - \hat{\mu}_1\right)^T \hat{\nabla} \left(X_i^\dagger - \hat{\mu}_1\right) - 2m\hat{\delta}^T \hat{\Sigma}_2^{-1}(\bar{X} - \hat{\mu}_1) + m\hat{\delta}^T \hat{\Sigma}_2^{-1}\hat{\delta} - m \log\left(\frac{\left|\hat{\Sigma}_1\right|}{\left|\hat{\Sigma}_2\right|}\right) + 2\log\left(\frac{\hat{\pi}_1}{\hat{\pi}_2}\right) < 0,$$

where $\hat{\delta} = \hat{\mu}_2 - \hat{\mu}_1$ and $\bar{X} = \sum_{i=1}^{m} X_i^\dagger / m$. Define

$$\hat{A}_{m,p} = \sum_{i=1}^{m} \left(X_i^\dagger - \hat{\mu}_1\right)^T \hat{\nabla} \left(X_i^\dagger - \hat{\mu}_1\right) - 2m\hat{\delta}^T \hat{\Sigma}_2^{-1}(\bar{X} - \hat{\mu}_1) := \hat{A}_{1,m,p} + \hat{A}_{2,m,p}.$$

Then the generalization error $\hat{R}_{1,m}$, which is a random variable as a function of $\{(\mathcal{X}_i, \mathcal{Y}_i)\}_{i=1}^N$, can be written as

$$\hat{R}_1 = \hat{R}_1((\mathcal{X}, \mathcal{Y})) = \mathrm{pr}\left(\hat{A}_{m,p} - \mathbb{E}\hat{A}_{m,p} < -\hat{\alpha}\right), \tag{S2.10}$$

where pr and $\mathbb{E}$ are understood as the conditional expectation given $\{(\mathcal{X}_i, \mathcal{Y}_i)\}_{i=1}^N$ and

$$\hat{\alpha} = \mathbb{E}(\hat{A}_{1,m,p} + \hat{A}_{2,m,p}) + m\hat{\delta}^T\hat{\Sigma}_2^{-1}\hat{\delta} - m\log\left(\left|\hat{\Sigma}_1\right| / \left|\hat{\Sigma}_2\right|\right) + 2\log\left(\frac{\hat{\pi}_1}{\hat{\pi}_2}\right).$$

The following lemma facilitates our analysis.

**Lemma 1.** *For any fixed $L > 0$, under the assumptions $p \leq c_0 N m_0$ and $\log p \leq c_0 N$ with sufficiently small $c_0 > 0$, we have that (i) $C'^{-1} \leq \lambda_{\min}(\hat{\Sigma}_k) \leq \lambda_{\max}(\hat{\Sigma}_k) \leq C'$; (ii) $\|\mu_k - \hat{\mu}_k\| \leq C'\sqrt{\frac{p}{Nm_0}}$; (iii) $\|\Sigma_k - \hat{\Sigma}_k\|_F \leq C'\sqrt{\frac{p^2}{Nm_0}}$ and (iv) $|\pi_k - \hat{\pi}_k| \leq C'\sqrt{\frac{\log p}{N}}$, $k = 1, 2$ with probability at least $1 - O(p^{-L})$, where positive constant $C'$ depend on $C_e, c_m, L$ and $C_\pi$ only.*

From now on, we condition on the event $\mathcal{E}$ in which results (i)-(iv) of Lemma 1 hold for training data $\{(\mathcal{X}_i, \mathcal{Y}_i)\}_{i=1}^N$. All positive constants used hereafter only depend on $C_e$ and $c_0$. Clearly, since $p^2/(Nm_0 D_p^2)$ is sufficiently small, Lemma 1 (ii) and (iii) imply that

$$\hat{D}_p = \left(\|\hat{\nabla}\|_F^2 + \|\hat{\delta}\|^2\right)^{1/2} \asymp D_p. \tag{S2.11}$$

We show the concentration radius of $\hat{A}_{m,p} - \mathbb{E}\hat{A}_{m,p}$ is much smaller than $\hat{\alpha}$ under our assumptions.

First of all, we analyze the left side $\hat{A}_{m,p} - \mathbb{E}\hat{A}_{m,p} = \Sigma_{k=1}^2(\hat{A}_{k,m,p} - \mathbb{E}\hat{A}_{k,m,p})$. Note that $\hat{A}_{2,m,p} - \mathbb{E}\hat{A}_{2,m,p} = -2\sum_{i=1}^m \hat{\delta}^T\hat{\Sigma}_2^{-1}\Sigma_1^{1/2}Z_i$, where $Z_i = \Sigma_1^{-1/2}(X_i^\dagger - \mu_1) \overset{\text{i.i.d}}{\sim} N(0, I)$. Note Lemma 1 implies the spectral norm $\left\|\hat{\Sigma}_2^{-1}\Sigma_1^{1/2}\right\|_{\ell_2} \leq C'C_e^{1/2}$. The tail probability of normal distribution implies (similarly as in equation (S2.6)) there exists some constant $C_1 > 0$ such

that,

$$\mathrm{pr}(|\hat{A}_{2,m,p} - \mathbb{E}\hat{A}_{2,m,p}| > t) \leq 2\exp\left(-\frac{C_1 t^2}{m\|\hat{\delta}\|^2}\right). \tag{S2.12}$$

Besides, $\hat{A}_{1,m,p} - \mathbb{E}\hat{A}_{1,m,p} = W_1 + W_2$, where

$$\begin{aligned} W_1 \; : \; &= \mathrm{tr}[\hat{\nabla}(\sum_{i=1}^{m}\left(X_i^{\dagger} - \mu_1\right)\left(X_i^{\dagger} - \mu_1\right)^T)] - \mathrm{tr}[\hat{\nabla} m\Sigma_1], \\ W_2 &:= 2\left(\mu_1 - \hat{\mu}_1\right)^T \hat{\nabla}\Sigma_1^{1/2}\sum_{i=1}^{m} Z_i. \end{aligned}$$

Set $\hat{V} = \Sigma_1^{1/2}\hat{\nabla}\Sigma_1^{1/2}$ and its eigen-values $\{\hat{\lambda}_j\}_{j=1}^{p}$. By a similar argument using Bernstein's inequality like (S2.7), we have that there exists some constant $c_1 > 0$ such that

$$\mathrm{pr}(|W_1| > t) \leq 2\exp\left(-c_1\min(\frac{t^2}{m\|\hat{V}\|_F^2}, \frac{t}{\max\{\left|\hat{\lambda}_1\right|, \left|\hat{\lambda}_p\right|\}})\right). \tag{S2.13}$$

To control $W_2$, we apply again the tail probability of normal distribution to obtain that for some constants $C_2$, $C_3 > 0$,

$$\mathrm{pr}(|W_2| > t) \leq 2\exp\left(-\frac{C_2 t^2}{m\|\hat{\nabla}\|_{\ell_2}^2 \cdot \|\mu_1 - \hat{\mu}_1\|^2}\right) \leq 2\exp\left(-\frac{C_3 t^2}{m\|\hat{\nabla}\|_F^2}\right), \tag{S2.14}$$

since $\|\mu_1 - \hat{\mu}_1\| \leq C'\sqrt{\frac{p}{Nm_0}} \leq C' c_0^{1/2}$ by Lemma 1. Therefore equations (S2.12)-(S2.14), together with (S2.11), imply that for some $C_4 > 0$,

$$\mathrm{pr}(|\hat{A}_{m,p} - \mathbb{E}\hat{A}_{m,p}| > t) \leq 6\exp\left(-\frac{C_4 t^2}{mD_p^2}\right). \tag{S2.15}$$

Now we lower bound the right side $\hat{\alpha}$. This term can be decomposed into six terms.

$$\begin{aligned} \hat{\alpha} \;=\; & m\hat{\delta}^T\hat{\Sigma}_2^{-1}\hat{\delta} + \left[m\mathrm{tr}(\hat{\nabla}\hat{\Sigma}_1) - m\log\left(\left|\hat{\Sigma}_1\right| / \left|\hat{\Sigma}_2\right|\right)\right] + 2\log\left(\frac{\hat{\pi}_1}{\hat{\pi}_2}\right) + \\ & m\mathrm{tr}(\hat{\nabla}(\Sigma_1 - \hat{\Sigma}_1)) - 2m\hat{\delta}^T\hat{\Sigma}_2^{-1}\left(\mu_1 - \hat{\mu}_1\right) + m\left(\mu_1 - \hat{\mu}_1\right)\hat{\nabla}\left(\mu_1 - \hat{\mu}_1\right)^T. \end{aligned}$$

These terms have the following bounds respectively with some constant $C_5, C_6, C_7, C_8, C_9 >$

0,

$$m\hat{\delta}^T\hat{\Sigma}_2^{-1}\hat{\delta} \geq C_5 m\|\hat{\delta}\|^2, \quad \text{(S2.16)}$$

$$m\mathrm{tr}(\hat{\nabla}\hat{\Sigma}_1) - m\log\left(\left|\hat{\Sigma}_1\right| / \left|\hat{\Sigma}_2\right|\right) \geq C_5 m\|\hat{\nabla}\|_F^2, \quad \text{(S2.17)}$$

$$\left|m\mathrm{tr}(\hat{\nabla}(\Sigma_1 - \hat{\Sigma}_1))\right| \leq C_6 m\|\hat{\nabla}\|_F\|\Sigma_1 - \hat{\Sigma}_1\|_F \leq C_7 m\|\hat{\nabla}\|_F(p^2/Nm_0)^{1/2}, \quad \text{(S2.18)}$$

$$\left|2m\hat{\delta}^T\hat{\Sigma}_2^{-1}(\mu_1 - \hat{\mu}_1)\right| \leq C_6 m\|\hat{\delta}\|\|\mu_1 - \hat{\mu}_1\| \leq C_7 m\|\hat{\delta}\|(p/Nm_0)^{1/2}, \quad \text{(S2.19)}$$

$$|2\log(\hat{\pi}_1/\hat{\pi}_2)| \leq C_6, \quad \text{(S2.20)}$$

$$\left|m(\mu_1 - \hat{\mu}_1)\hat{\nabla}(\mu_1 - \hat{\mu}_1)^T\right| \leq C_8 m\|\hat{\nabla}\|_{\ell_2}\|\mu_1 - \hat{\mu}_1\|^2 \leq C_9 m(p/Nm_0). \quad \text{(S2.21)}$$

Equations (S2.16) and (S2.17) are due to (i) of Lemma 1. In particular, (S2.17) follows from a similar argument as (S2.8). Equations (S2.18) and (S2.19) follow from (iii) and (ii) of Lemma 1 respectively while equation (S2.20) is due to (iv) of Lemma 1 and Condition 3. Equation (S2.21) follows from (i) and (ii) of Lemma 1. Furthermore, notice that $p^2/(Nm_0D_p^2)$ is sufficiently small and $m_0D_p^2$ is sufficiently large, equations (S2.16)-(S2.21) as well as (S2.11) yield that $\hat{\alpha} \geq C_{10}mD_p^2$ for some small constant $C_{10} > 0$.

Finally, the lower bound of $\hat{\alpha}$ and concentration of $\hat{A}_{m,p} - \mathbb{E}\hat{A}_{m,p}$ in (S2.15) with $t = c''mD_p^2$ for small enough $c'' > 0$, together with the assumption $D_p^2 m$ is sufficiently large, imply that the generalization error of the quadratic set classification rule $\hat{R}_{1,m} \leq 2\exp\left(-c'mD_p^2\right)$ for each $m \in [c_m m_0, C_m m_0]$ on the event $\mathcal{E}$. Hence we complete our proof by applying Lemma 1 and equation (S2.9), that is, $\hat{R} \leq 4\exp\left(-c'm_0D_p^2\right)$ with probability at least $1 - O(p^{-L})$. □

### Proof of Theorem 3

*Proof.* First we show that $\Sigma_k^{-1}$ is feasible for the optimization problem (3.7), that is $\|\hat{\Sigma}_k\Sigma_k^{-1} - I\|_\infty < \lambda_{1,N}$. It suffices to show that $\|\hat{\Sigma}_k - \Sigma_k\|_\infty < C_{\ell 1}^{-1}\lambda_{1,N}$ because $\|\hat{\Sigma}_k\Sigma_k^{-1} - I\|_\infty \leq$

$\|\hat{\Sigma}_k - \Sigma_k\|_\infty \|\Sigma_k^{-1}\|_{\ell_1} \leq \|\hat{\Sigma}_k - \Sigma_k\|_\infty C_{\ell 1}$. The following lemma establishes this result, given our choice of $\lambda_{1,N} \geq CC_{\ell 1}\sqrt{(\log p)/(Nm_0)}$ and the assumption $\log p \leq c_0 N$ with some sufficiently small $c_0 > 0$.

**Lemma 2.** *Recall the number of set from class $k$ is denoted as $N_k = \sum_{i=1}^N \mathbb{1}\{\mathcal{Y}_i = k\}$. Then given any positive integer $N_1$ and $N_2$, we have that with probability at least $1 - O(p^{-L})$ (i) $\|\hat{\mu}_k - \mu_k\|_\infty \leq C'\sqrt{(\log p)/(N_k m_0)}$ and (ii) $\|\hat{\Sigma}_k - \Sigma_k\|_\infty \leq C'(\sqrt{(\log p)/(N_k m_0)} + (\log p)/(N_k m_0))$, $k = 1, 2$, where positive constant $C'$ depends on $C_e, c_m$ and $L$ only. Under the assumption $\log p \leq c_0 N$ with some sufficiently small $c_0 > 0$, we further have that (i) $\|\hat{\mu}_k - \mu_k\|_\infty \leq C\sqrt{(\log p)/(Nm_0)}$ and (ii) $\|\hat{\Sigma}_k - \Sigma_k\|_\infty \leq C\sqrt{(\log p)/(Nm_0)}$, $k = 1, 2$ with probability at least $1 - O(p^{-L})$, where the constant $C$ also depends $C_\pi$ besides $C_e, c_m, L$.*

From now on, we condition on the event in which both results of the second part in Lemma 2 hold. We next control the supnorm bound $\left\|\Sigma_k^{-1} - \tilde{\Omega}_k\right\|_\infty$. Since both $\Sigma_k^{-1}$ and $\tilde{\Omega}_k$ are feasible for (3.7), we have $\|\hat{\Sigma}_k(\Sigma_k^{-1} - \tilde{\Omega}_k)\|_\infty = \|\hat{\Sigma}_k\Sigma_k^{-1} - I - (\hat{\Sigma}_k\tilde{\Omega}_k - I)\|_\infty \leq 2\lambda_{1,N}$. Moreover,

$$
\begin{aligned}
\|\Sigma_k(\Sigma_k^{-1} - \tilde{\Omega}_k)\|_\infty &\leq \|(\hat{\Sigma}_k - \Sigma_k)(\Sigma_k^{-1} - \tilde{\Omega}_k)\|_\infty + \|\hat{\Sigma}_k(\Sigma_k^{-1} - \tilde{\Omega}_k)\|_\infty \\
&\leq \|\Sigma_k^{-1} - \tilde{\Omega}_k\|_{\ell_1}\|\hat{\Sigma}_k - \Sigma_k\|_\infty + 2\lambda_{1,N} \\
&\leq \left(\left\|\Sigma_k^{-1}\right\|_{\ell_1} + \|\tilde{\Omega}_k\|_{\ell_1}\right) C_{\ell 1}^{-1}\lambda_{1,N} + 2\lambda_{1,N} \\
&\leq 2C_{\ell 1}C_{\ell 1}^{-1}\lambda_{1,N} + 2\lambda_{1,N} = 4\lambda_{1,N},
\end{aligned}
$$

where we have used the fact $\tilde{\Omega}_k$ is the solution of CLIME which implies for each $j = 1, \ldots, p$, $\|(\tilde{\Omega}_k)_j\|_1 \leq \left\|(\Sigma_k^{-1})_j\right\|_1$ and hence $\|\tilde{\Omega}_k\|_{\ell_1} \leq \left\|\Sigma_k^{-1}\right\|_{\ell_1}$, where $(\tilde{\Omega}_k)_j$ and $(\Sigma_k^{-1})_j$ denote the $j$th column of $\tilde{\Omega}_k$ and $\Sigma_k^{-1}$ respectively. We conclude with $\|\Sigma_k^{-1} - \tilde{\Omega}_k\|_\infty \leq \|\Sigma_k^{-1}\|_{\ell_1}\|\Sigma_k(\Sigma_k^{-1} - \tilde{\Omega}_k)\|_\infty \leq 4M_0\lambda_{1,N}$.

Based on the supnorm bound obtained above, we have

$$\|(\tilde{\Omega}_2 - \tilde{\Omega}_1) - \nabla\|_\infty \le \|\Sigma_1^{-1} - \tilde{\Omega}_1\|_\infty + \|\Sigma_2^{-1} - \tilde{\Omega}_2\|_\infty \le 8C_{\ell 1}\lambda_{1,N}. \tag{S2.22}$$

Recall that $\mathrm{supp}(\nabla)$ is the support of the matrix $\nabla$. The thresholding step (3.8), together with (S2.22), guarantees that $\tilde{\nabla}_{ij} = 0$ for any $(i,j) \notin \mathrm{supp}(\nabla)$, noting that $\lambda'_{1,N} \ge 8C_{\ell 1}\lambda_{1,N}$. Therefore we have shown the subset selection result, that is, $\mathrm{pr}(\mathrm{supp}(\tilde{\nabla}) \subset \mathrm{supp}(\nabla)) = 1 - O(p^{-L})$. Moreover, we have that $\|\tilde{\nabla} - \nabla\|_\infty \le 8C_{\ell 1}\lambda_{1,N} + \lambda'_{1,N} \le 2\lambda'_{1,N}$. In the end, we complete the proof by noting that the Frobenius norm bound and vector $\ell_1$ norm bound are the consequences of supnorm bound and subset selection result, that is, $\mathrm{pr}(\|\tilde{\nabla} - \nabla\|_F \le 2\lambda'_{1,N}\sqrt{s_q}) = 1 - O(p^{-L})$ and $\mathrm{pr}(\|\tilde{\nabla} - \nabla\|_1 \le 2\lambda'_{1,N}s_q) = 1 - O(p^{-L})$. □

**Proof of Theorem 4**

*Proof.* We first show that $(\beta_1, \beta_2) = (\Sigma_1^{-1}\mu_1, \Sigma_2^{-1}\mu_2)$ is feasible in (3.9) with the constant $L_1$ set as $C_\beta$. Note since $\|\beta_k\|_1 \le C_\beta$, The pair $(\beta_1, \beta_2)$ satisfies the $\ell_1$ norm constraint. This fact, together with the following lemma, implies that $(\beta_1, \beta_2)$ is feasible with probability at least $1 - O(p^{-L})$ and hence $\|\hat{\beta}\|_1 \le \|\beta\|_1$.

**Lemma 3.** *Under the assumption* $\log p \le c_0 N$ *with some sufficiently small constant* $c_0 > 0$*, we have that* $\mathrm{pr}(\|\hat{\Sigma}_k\beta_k - \hat{\mu}_k\|_\infty \ge C\sqrt{\frac{\log p}{Nm_0}}) \le C'p^{-L}$, $k = 1, 2$, *where* $C' > 0$ *is some universal constant and constant* $C > 0$ *depends on* $C_e, c_m, C_\pi, C_\beta, C_\mu$ *and* $L$ *only.*

Next we show that $\|\tilde{\beta} - \beta\|_\infty \le 6C_{\ell 1}\lambda_{2,N}$. Notice that for $k = 1, 2$, there exists some

constant $C > 0$ such that with probability at least $1 - O(p^{-L})$,

$$\begin{aligned}\|\Sigma_k\left(\tilde{\beta}_k - \beta_k\right)\|_\infty &\leq \|\hat{\Sigma}_k\left(\tilde{\beta}_k - \beta_k\right)\|_\infty + \|\left(\Sigma_k - \hat{\Sigma}_k\right)\left(\tilde{\beta}_k - \beta_k\right)\|_\infty \\ &\leq \|\hat{\Sigma}_k\beta_k - \hat{\mu}_k\|_\infty + \|\hat{\Sigma}_k\tilde{\beta}_k - \hat{\mu}_k\|_\infty + \|\Sigma_k - \hat{\Sigma}_k\|_\infty\left(\|\beta_k\|_1 + \|\tilde{\beta}_k\|_1\right) \\ &\leq 2\lambda_{2,N} + 2C_\beta C\sqrt{\frac{\log p}{Nm_0}} \leq 3\lambda_{2,N},\end{aligned}$$

where we have used assumption on $\|\beta_k\|_1$, constraints on estimators, the choice of our $\lambda_{2,N}$ and the result (ii) of the second part in Lemma 2. Therefore we further have,

$$\|\tilde{\beta} - \beta\|_\infty \leq \sum_{k=1}^{2}\|\tilde{\beta}_k - \beta_k\|_\infty \leq \sum_{k=1}^{2}\|\Sigma_k^{-1}\|_{\ell_1}\|\Sigma_k\left(\tilde{\beta}_k - \beta_k\right)\|_\infty \leq 6C_{\ell 1}\lambda_{2,N}. \tag{S2.23}$$

In the end, we condition on the event in which both (S2.23) and the fact that $(\beta_1, \beta_2)$ is feasible hold. The arguments above imply this event holds with probability at least $1 - O(p^{-L})$. We are ready to prove the rates of convergence of $\tilde{\beta}$ under $\ell_1$ and $\ell_2$ norm losses. Denote the support of $\beta$ by $T$. Set $t = 6C_{\ell 1}\lambda_{2,N}$ and the thresholded version of $\tilde{\beta}$ as $\tilde{\beta}^{thr} = (\tilde{\beta}_j^{thr})$, where $\tilde{\beta}_j^{thr} = \tilde{\beta}_j\mathbb{1}\left\{|\tilde{\beta}_j| \geq 2t\right\}$. Since $\beta = \beta_1 - \beta_2$ is feasible, we have that $\|\beta\|_1 \geq \|\tilde{\beta}\|_1 = \|\tilde{\beta}^{thr}\|_1 + \|\tilde{\beta} - \tilde{\beta}^{thr}\|_1 \geq \|\tilde{\beta} - \tilde{\beta}^{thr}\|_1 + \|\beta\|_1 - \|\tilde{\beta}^{thr} - \beta\|_1$. Therefore we obtain that $\|\tilde{\beta} - \tilde{\beta}^{thr}\|_1 \leq \|\tilde{\beta}^{thr} - \beta\|_1$, which further implies that $\|\tilde{\beta} - \beta\|_1 \leq 2\|\tilde{\beta}^{thr} - \beta\|_1$. To show the bound of $\|\tilde{\beta} - \beta\|_1$, it suffices to bound $\|\tilde{\beta}^{thr} - \beta\|_1$. Indeed, we bound its $\ell_2$ norm as an intermediate step,

$$\begin{aligned}\|\tilde{\beta}^{thr} - \beta\|^2 &= \|\left(\tilde{\beta}^{thr} - \beta\right)_T\|^2 \\ &= \sum_{j\in T}\left(\tilde{\beta}_j^{thr} - \beta_j\right)^2\mathbb{1}\left\{\tilde{\beta}_j^{thr} = 0\right\} + \sum_{j\in T}\left(\tilde{\beta}_j - \beta_j\right)^2\mathbb{1}\left\{\tilde{\beta}_j^{thr} \neq 0\right\} \\ &\leq \sum_{j\in T}\beta_j^2\mathbb{1}\{\beta_j \leq 3t\} + s_l t^2 \leq 10 s_l t^2,\end{aligned} \tag{S2.24}$$

where we have used supnorm bound (S2.23) in the first and third equations and the fact

$|T| \leq s_l$ due to $\beta \in \mathcal{F}_0(s_l)$ in the third and fourth equations. Consequently,

$$\|\tilde{\beta}^{thr} - \beta\|_1 = \| \left(\tilde{\beta}^{thr} - \beta\right)_T \|_1 \leq \sqrt{s_l}\|\tilde{\beta}^{thr} - \beta\| = \sqrt{10}s_l t,$$

which completes our first desired result $\|\tilde{\beta} - \beta\|_1 \leq 2\sqrt{10}s_l t = 12\sqrt{10}C_{\ell 1}s_l\lambda_{2,N}$.

To show the bound of $\|\tilde{\beta} - \beta\| \leq \|\tilde{\beta}^{thr} - \beta\| + \|\tilde{\beta} - \tilde{\beta}^{thr}\|$, it suffices to bound $\|\tilde{\beta} - \tilde{\beta}^{thr}\|$ given (S2.24). To this end, we note $\|\beta\|_1 \geq \|\tilde{\beta}\|_1$ implies that $\|\tilde{\beta}_{T^c}\|_1 \leq \|\tilde{\beta} - \beta\|_1 \leq 2\sqrt{10}s_l t$. Moreover,

$$\begin{aligned} \|\tilde{\beta} - \tilde{\beta}^{thr}\|^2 &= \| \left(\tilde{\beta}^{thr} - \tilde{\beta}\right)_T \|^2 + \| \left(\tilde{\beta}^{thr} - \tilde{\beta}\right)_{T^c} \|^2 \\ &\leq 4t^2 s_l + \sum_{j \in T^c} \tilde{\beta}_j^2 \mathbb{1}\left\{|\tilde{\beta}_j| < 2t\right\} \\ &\leq 4t^2 s_l + \|\tilde{\beta}_{T^c}\|_1 \max_{j \in T^c}\{|\tilde{\beta}_j| \mathbb{1}\left\{|\tilde{\beta}_j| < 2t\right\}\} \leq (4 + 4\sqrt{10})t^2 s_l, \quad \text{(S2.25)} \end{aligned}$$

where the first inequality follows from $|\tilde{\beta}_j^{thr} - \tilde{\beta}_j| < 2t$ and $|T| \leq s_l$, and the second one is due to Hölder's inequality. Therefore combining (S2.24) and (S2.25), we obtained the second desired result $\|\tilde{\beta} - \beta\| \leq \sqrt{s_l}t(\sqrt{10} + (4 + 4\sqrt{10})^{1/2})$. □

### Proof of Theorem 5

*Proof.* Since we use sample splitting technique, estimators $\tilde{\beta}$ and $\tilde{\nabla}$ are independent with the second batch of the training data used in (3.10). We assume fixed $\tilde{\beta}$ and $\tilde{\nabla}$, which satisfy our assumptions throughout the analysis. With a slight abuse of notation, we still use $N$ to denote the number of sample sets, although only half of the sample sets are applied to count $n_k$ and $\hat{\pi}_k$, $k = 1, 2$.

Recall that $\bar{X}_i$ and $S_i$ are the sample mean and variance of the $i$th set of observations. Define $\tilde{Z}_i = \log(\hat{\pi}_1/\hat{\pi}_2)/M_i + \bar{X}_i^T\tilde{\beta} + \bar{X}_i^T\tilde{\nabla}\bar{X}_i/2 + \text{tr}(\tilde{\nabla}S_i)/2$, which is used to approximate $Z_i = \log(\pi_1/\pi_2)/M_i + \bar{X}_i^T\beta + \bar{X}_i^T\nabla\bar{X}_i/2 + \text{tr}(\nabla S_i)/2$. To facilitate analysis, we denote

$\ell(\theta_0|\{(\mathcal{X}_i, \mathcal{Y}_i)\}_{i=1}^N, \tilde{\beta}, \tilde{\nabla})$ as $\ell(\theta_0)$ for short. Rewrite our estimator in the following way,

$$\begin{aligned}\tilde{\beta}_0 &= \operatorname*{argmin}_{\theta_0 \in \mathbb{R}} \ell(\theta_0), \text{where} \\ \ell(\theta_0) &= \frac{1}{N}\Sigma_{i=1}^N[\log\left(1+\exp(M_i(\theta_0+\tilde{Z}_i))\right) - (2-\mathcal{Y}_i)M_i\left(\theta_0+\tilde{Z}_i\right)].\end{aligned}$$

We start our analysis by conditioning on $\{\mathcal{X}_i\}_{i=1}^N$. Define $\ell_0(\theta_0, \tilde{Z}) = \mathbb{E}(\ell(\theta_0)|\{\mathcal{X}_i\}_{i=1}^N)$ where the expectation is understood as the conditional expectation given $\{\mathcal{X}_i\}_{i=1}^N$. Note that the function $\ell_0(\theta_0, \tilde{Z})$ depends on $\theta_0, \{M_i\}_{i=1}^N$ and $\{\tilde{Z}_i\}_{i=1}^N$ only. Then the difference $\ell(\theta_0) - \ell_0(\theta_0, \tilde{Z}) = \frac{1}{N}\Sigma_{i=1}^N(\mathcal{Y}_i - \mathbb{E}(\mathcal{Y}_i|\mathcal{X}_i))M_i(\theta_0+\tilde{Z}_i) := E_{\theta_0}$. Recall $\beta_0$ is the true constant coefficient. Since $\tilde{\beta}_0$ is the minimizer, we have $\ell(\tilde{\beta}_0) \leq \ell(\beta_0)$, i.e.,

$$\begin{aligned}\ell_0(\tilde{\beta}_0, \tilde{Z}) &\leq \ell_0(\beta_0, \tilde{Z}) + E_{\beta_0} - E_{\tilde{\beta}_0} \\ &\leq \ell_0(\beta_0, \tilde{Z}) + m_0 R_1 \left|\tilde{\beta}_0 - \beta_0\right|. \qquad \text{(S2.26)}\end{aligned}$$

In the end, we need to bound the term $R_1 = |\frac{1}{Nm_0}\Sigma_{i=1}^N(\mathcal{Y}_i - \mathbb{E}(\mathcal{Y}_i|\mathcal{X}_i))M_i|$. By applying Hoeffding's inequality (e.g. Vershynin, 2012, Proposition 5.10), we obtain $R_1 \leq C_r\sqrt{(\log p)/N}$ with probability at least $1 - O(p^{-L})$, where constant $C_r$ depends on $L$ and $C_m$ only, noting that $M_i \leq C_m m_0$ by Condition 2. This probabilistic statement on bounding $R_1$ is valid conditioning on any realization of $\{\mathcal{X}_i\}_{i=1}^N$ and thus is also valid unconditionally.

Next we apply the Taylor expansion to the function $\ell_0(\theta_0, \tilde{Z})$ to analyze our estimator. Here due to misspecified values $\tilde{Z}_i$, we need a refined version of Taylor expansion (Bach et al., 2010, Proposition 1).

**Lemma 4** (Bach et al. (2010)). *Let $g(t) : \mathbb{R} \to \mathbb{R}$ be a convex three times differentiable function such that it satisfies for all $t \in \mathbb{R}$, $|g'''(t)| \leq Lg''(t)$ for some $L > 0$. Then we have*

*for any $t$ and $v \in \mathbb{R}$,*

$$g(t+v) \geq g(t) + vg'(t) + \frac{g''(t)}{L^2}(e^{-L|v|} + L\,|v| - 1).$$

It is not hard to see that the third derivative of $\ell_0(\theta_0, \tilde{Z})$ w.r.t. $\theta_0$ is bounded by its second derivative up to a multiplicative factor $\max_i M_i$, i.e.,

$$\max_{\theta_0} \left| \ell_0'''(\theta_0, \tilde{Z}) / \ell_0''(\theta_0, \tilde{Z}) \right| \leq \max_i M_i,$$

where hereafter $\ell_0'(\cdot,\cdot)$, $\ell_0''(\cdot,\cdot)$ and $\ell_0'''(\cdot,\cdot)$ are defined as the first, second and third derivative of $\ell_0(\cdot,\cdot)$ w.r.t. the first argument respectively. Applying Lemma 4 to $\ell_0(\theta_0, \tilde{Z})$ at point $\beta_0$ and by Condition 2, we obtain that

$$\ell_0(\tilde{\beta}_0, \tilde{Z}) - \ell_0(\beta_0, \tilde{Z}) \geq \ell_0'(\beta_0, \tilde{Z})(\tilde{\beta}_0 - \beta_0) + \frac{\ell_0''(\beta_0, \tilde{Z})}{C_m^2 m_0^2}(e^{-C_m m_0 \left|\tilde{\beta}_0 - \beta_0\right|} + C_m m_0 \left|\tilde{\beta}_0 - \beta_0\right| - 1). \tag{S2.27}$$

Note that with misspecified values $\tilde{Z}_i$, in general $\ell_0'(\beta_0, \tilde{Z}) \neq 0$. To finish our proof, we need an upper bound for $\ell_0'(\beta_0, \tilde{Z})$ and a lower bound for $\ell_0''(\beta_0, \tilde{Z})$ with misspecified values $\tilde{Z}_i$. Thus the term $|\tilde{Z}_i - Z_i|$ critically determines the estimation accuracy. The following bound of $|\tilde{Z}_i - Z_i|$ is helpful for our later analysis.

**Lemma 5.** *Under the assumptions of Theorem 5, there exists some constant $C_z > 0$ depending on $c_m, C_m, C_\pi, C_\mu$ and $C_e$ such that with probability at least $1 - O(p^{-L})$ we have uniformly for all $i = 1, \ldots, N$*

$$\begin{aligned} \left|\tilde{Z}_i - Z_i\right| &\leq \frac{1}{M_i}\left|\log\left(\frac{\hat{\pi}_1 \pi_2}{\hat{\pi}_2 \pi_1}\right)\right| + \left|\bar{X}_i^T\left(\tilde{\beta} - \beta\right)\right| + \frac{1}{M_i}\left|\sum_{j=1}^{M_i} X_{ij}^T\left(\tilde{\nabla} - \nabla\right)X_{ij}/2\right| \\ &\leq C_z\left((1 + \sqrt{\frac{\log p}{m_0}})\|\tilde{\beta} - \beta\| + (1 + \frac{\log p}{m_0})\|\tilde{\nabla} - \nabla\|_1 + \max_{k=1,2}\frac{|\pi_k - \hat{\pi}_k|}{m_0}\right) \end{aligned} \tag{S2.28}$$

*Indeed, the conclusion (S2.28) is valid with the same probability $1 - O(p^{-L})$ conditioning on any realization of $\{\mathcal{Y}_i\}_{i=1}^N$ and $\{M_i\}_{i=1}^N$.*

Lemma 5 and our assumption imply that with probability at least $1 - O(p^{-L})$ we have $m_0 \max_i |\tilde{Z}_i - Z_i| := R_2$ is sufficiently small.

Note that the expectation of the score function $\ell_0'(\beta_0, Z) = 0$ where $\ell_0'(\beta_0, Z)$ is obtained by replacing $\tilde{Z}_i$ by $Z_i$ in $\ell_0'(\beta_0, \tilde{Z})$, $i = 1, \ldots, N$. We are ready to bound the magnitude of $\ell_0'(\beta_0, \tilde{Z})$,

$$\begin{aligned} \left|\ell_0'(\beta_0, \tilde{Z})\right| &= \left|\frac{1}{N}\Sigma_{i=1}^N \left(\frac{M_i \exp(M_i(\beta_0 + \tilde{Z}_i))}{1 + \exp(M_i(\beta_0 + \tilde{Z}_i))} - \frac{M_i \exp(M_i(\beta_0 + Z_i))}{1 + \exp(M_i(\beta_0 + Z_i))}\right)\right| \\ &\leq \frac{1}{N}\Sigma_{i=1}^N M_i^2 \left|\tilde{Z}_i - Z_i\right| \\ &\leq C_m^2 m_0 R_2, \end{aligned} \tag{S2.29}$$

where the first inequality follows from that the derivative of $\frac{\exp(M_i(\beta_0+\tilde{Z}_i))}{1+\exp(M_i(\beta_0+\tilde{Z}_i))}$ w.r.t. $\tilde{Z}_i$ is always bounded by $M_i$ and the second inequality is due to Condition 2, $M_i \leq C_m m_0$ and definition of $R_2$.

Moreover, by Condition 4, we have that the expectation of the i.i.d. bounded random variable $\mathrm{Var}(\mathcal{Y}_i \mid \mathcal{X}_i) = \frac{\exp(M_i(\beta_0+Z_i))}{(1+\exp(M_i(\beta_0+Z_i)))^2}$, $i = 1, \ldots, N$, is bounded away from $C_{\log}$. We apply Hoeffding's inequality and the fact $\log p \leq c_0 N$ to obtain that with probability at least $1 - O(p^{-L})$, we have

$$\frac{1}{N}\Sigma_{i=1}^N M_i^2 \left(\frac{\exp(M_i(\beta_0 + Z_i))}{1 + \exp(M_i(\beta_0 + Z_i))}\right)\left(\frac{1}{1 + \exp(M_i(\beta_0 + Z_i))}\right) \geq C_{low}' m_0^2,$$

where the positive constant $C_{low}' > 0$ depends on $C_{\log}$ and $L$. Since $m_0 \max_i |\tilde{Z}_i - Z_i| := R_2$ is sufficiently small with probability at least $1 - O(p^{-L})$, the union bound argument further implies that

$$\begin{aligned} \ell_0''(\beta_0, \tilde{Z}) &= \frac{1}{N}\Sigma_{i=1}^N M_i^2 \left(\frac{\exp\left(M_i(\beta_0 + \tilde{Z}_i)\right)}{1 + \exp\left(M_i(\beta_0 + \tilde{Z}_i)\right)}\right)\left(\frac{1}{1 + \exp\left(M_i(\beta_0 + \tilde{Z}_i)\right)}\right) \\ &\geq C_{low} m_0^2, \end{aligned} \tag{S2.30}$$

with probability at least $1 - O(p^{-L})$ for some positive constant $C_{low} > 0$.

In the end, plugging (S2.26), (S2.29) and (S2.30) into (S2.27) and applying the union bound argument, we obtain that with probability $1 - O(p^{-L})$,

$$C_{low}C_m^{-2}(e^{-C_m m_0 |\tilde{\beta}_0 - \beta_0|} + C_m m_0 \left|\tilde{\beta}_0 - \beta_0\right| - 1) \leq m_0 \left(C_m^2 R_2 + R_1\right) \left|\tilde{\beta}_0 - \beta_0\right|. \qquad \text{(S2.31)}$$

We apply the following fact

$$e^{-2\gamma/(1-\gamma)} + (1-\gamma)\frac{2\gamma}{1-\gamma} - 1 \geq 0 \text{ for } \gamma \in (0,1),$$

to (S2.31) and obtain that

$$C_m m_0 \left|\tilde{\beta}_0 - \beta_0\right| \leq \frac{2C_m(C_m^2 R_2 + R_1)/C_{\log}}{1 - C_m(C_m^2 R_2 + R_1)/C_{\log}}.$$

Since $C_m^2 R_2 + R_1$ are sufficiently small, we have that $C_m(C_m^2 R_2 + R_1)/C_{\log} < 1/2$ which implies $C_m m_0 |\tilde{\beta}_0 - \beta_0| < 2$. This fact itself further implies that $(e^{-C_m m_0 |\tilde{\beta}_0 - \beta_0|} + C_m m_0 |\tilde{\beta}_0 - \beta_0| - 1) \geq (C_m m_0 |\tilde{\beta}_0 - \beta_0|)^2/2$. Consequently, (S2.31) implies that

$$\left|\tilde{\beta}_0 - \beta_0\right| \leq 2C_{low}^{-1} m_0^{-1} \left(C_m^2 R_2 + R_1\right),$$

which further completes our proof, together with Lemma 5 (bound of $R_2$) and the bound of $R_1$,

$$\left|\tilde{\beta}_0 - \beta_0\right| \leq C_\delta \left( (1 + \sqrt{\frac{\log p}{m_0}}) \|\tilde{\beta} - \beta\| + (1 + \frac{\log p}{m_0}) \|\tilde{\nabla} - \nabla\|_1 + \max_{k=1,2} \frac{|\pi_k - \hat{\pi}_k|}{m_0} + \sqrt{\frac{\log p}{N m_0^2}} \right),$$

where the constant $C_\delta = 2C_{low}^{-1}(C_m^2 C_z + C_r)$. □

**Proof of Theorem 6**

*Proof.* Recall that for each $k = 1, 2$, the corresponding Bayes risk and generalization error of CLIPS classifier can be decomposed as

$$
\begin{aligned}
R_{Bk} &= \sum_{m=c_m m_0}^{C_m m_0} \mathrm{pr}(\phi_B(\mathcal{X}^\dagger) \neq k \mid \mathcal{Y}^\dagger = k, M^\dagger = m) p_M(m) := \sum_m R_{Bk,m} p_M(m), \\
\tilde{R}_k &= \sum_{m=c_m m_0}^{C_m m_0} \mathrm{pr}(\tilde{\phi}(\mathcal{X}^\dagger) \neq k \mid \mathcal{Y}^\dagger = k, M^\dagger = m) p_M(m) := \sum_m \tilde{R}_{k,m} p_M(m).
\end{aligned}
$$

Therefore, it is sufficient to bound the difference $\tilde{R}_{k,m} - R_{Bk,m}$ for each fixed $k = 1, 2$ and fixed $m \in [c_m m_0, C_m m_0]$.

Recall that $\Xi_N = (1 + \sqrt{\frac{\log p}{m_0}})\|\tilde{\beta} - \beta\| + (1 + \frac{\log p}{m_0})\|\tilde{\nabla} - \nabla\|_1 + \max_{k=1,2} \frac{|\hat{\pi}_k - \pi_k|}{m_0} + |\tilde{\beta}_0 - \beta_0|$. Define the event $\mathcal{E}_0 = \{\Xi_N \leq C_\Xi \kappa_N\}$, where $\kappa_N = (1 + \frac{\log p}{m_0}) s_q \lambda'_{1,N} + (1 + \sqrt{\frac{\log p}{m_0}}) C_{\ell 1} \sqrt{s_l} \lambda_{2,N} + \sqrt{\frac{\log p}{N m_0^2}}$, the constant $C_\Xi = 2(2 + C'')(C_\delta + 1)$ and other constants $C''$, $C_\delta$ can be tracked back from Theorems 3-5. We first show that our estimators satisfy that $\mathrm{pr}(\mathcal{E}_0) = 1 - O(p^{-L})$ by Theorems 3-5. Indeed, Theorems 3 and 4 provides bounds of $\|\tilde{\beta} - \beta\|$ and $\|\tilde{\nabla} - \nabla\|_1$ respectively. The estimation error of $\max_{k=1,2} |\hat{\pi}_k - \pi_k|/m_0$ follows from Lemma 1. Assuming these bounds hold, the first part of Condition 5 implies that the assumption in Theorem 5 is satisfied with the initial estimators being our quadratic and linear estimators. Thus Theorem 5 further implies the upper bound for $|\tilde{\beta}_0 - \beta_0|$. Hereafter, we assume event $\mathcal{E}_0$ holds.

We follow the notation introduced in the proof of Theorem 5 on the set of observations $(\mathcal{X}^\dagger, \mathcal{Y}^\dagger)$ and define $\tilde{Z} = \log(\hat{\pi}_1/\hat{\pi}_2)/M^\dagger + \bar{x}^T\tilde{\beta} + \bar{x}^T\tilde{\nabla}\bar{x}/2 + \mathrm{tr}(\tilde{\nabla}S)/2$, which is used to approximate $Z = \log(\pi_1/\pi_2)/M^\dagger + \bar{x}^T\beta + \bar{x}^T\nabla\bar{x}/2 + \mathrm{tr}(\nabla S)/2$, where $\bar{x}$ and $S$ are the sample mean and covariance of the set $\mathcal{X}^\dagger$. Then we define the event $\mathcal{E}_z = \{|\tilde{Z} - Z| \leq C_z \Xi_N\}$. Lemma 5 applied to $(\mathcal{X}^\dagger, \mathcal{Y}^\dagger)$ and the second part of Condition 5 imply that on event $\mathcal{E}_0$ uniformly for all $k = 1, 2$ and $m \in [c_m m_0, C_m m_0]$, we have $\mathrm{pr}(\mathcal{E}_z | \mathcal{Y}^\dagger = k, M^\dagger = m) \geq 1 - C'_g p^{-L}$.

Without loss of generality, we focus on the case $k = 1$. Recall $\tilde{R}_{k,m}$ relies on the estimators $\tilde{\beta}_0, \tilde{\beta}, \tilde{\nabla}, \hat{\pi}_1$ and $\hat{\pi}_2$ and hence is random. On the event $\mathcal{E}_0$, we have that

$$\begin{aligned}
\tilde{R}_{1,m} &= \mathrm{pr}\left(\tilde{Z} + \tilde{\beta}_0 \le 0 | \mathcal{Y}^\dagger = 1, M^\dagger = m\right) \\
&= \mathrm{pr}\left(Z + \beta_0 \le Z - \tilde{Z} + \beta_0 - \tilde{\beta}_0 | \mathcal{Y}^\dagger = 1, M^\dagger = m\right) \\
&= \mathrm{pr}\left(Z + \beta_0 \le Z - \tilde{Z} + \beta_0 - \tilde{\beta}_0, \mathcal{E}_z | \mathcal{Y}^\dagger = 1, M^\dagger = m\right) + \mathrm{pr}(\mathcal{E}_z^c | \mathcal{Y}^\dagger = 1, M^\dagger = m) \\
&\le C_g' p^{-L} + \mathrm{pr}\left(Z + \beta_0 \le (C_z + 1)\, \Xi_N, \mathcal{E}_z | \mathcal{Y}^\dagger = 1, M^\dagger = m\right) \\
&\le C_g' p^{-L} + \mathrm{pr}\left(Z + \beta_0 \le (C_z + 1)\, C_\Xi \kappa_N | \mathcal{Y}^\dagger = 1, M^\dagger = m\right) \\
&= C_g' p^{-L} + F_{1,m}((C_z + 1)\, C_\Xi \kappa_N), \qquad \text{(S2.32)}
\end{aligned}$$

where the first inequality follows from the conditional probability $\mathrm{pr}(\mathcal{E}_z | \mathcal{Y}^\dagger = k, M^\dagger = m) \ge 1 - C_g' p^{-L}$ and the definition of the event $\mathcal{E}_z$, the second inequality is due to the event $\mathcal{E}_0$, and the last equality follows from the definition of the cumulative distribution function $F_{1,m}(t)$.

In addition, by the definition of the deterministic value $R_{Bk,m}$, we have

$$R_{B1,m} = \mathrm{pr}\left(Z + \beta_0 \le 0 | \mathcal{Y}^\dagger = 1, M^\dagger = m\right) = F_{1,m}(0). \qquad \text{(S2.33)}$$

By our assumption, the quantity $(C_z + 1)\, C_\Xi \kappa_N$ is sufficiently small and hence less than $\delta_0$. It follows from (S2.32)-(S2.33) and definition of $d_N$ that on the event $\mathcal{E}_0$, we have that

$$\begin{aligned}
\tilde{R}_{1,m} - R_{B1,m} &\le C_g' p^{-L} + \sup_{t \in [-\delta_0, \delta_0]} \left| F_{1,m}'(t) \right| (C_z + 1)\, C_\Xi \kappa_N \\
&\le C_g' p^{-L} + (C_z + 1)\, C_\Xi \kappa_N d_N.
\end{aligned}$$

Similarly we can show that same upper bound applies to $\tilde{R}_{2,m} - R_{B2,m}$ uniformly for all $m \in [c_m m_0, C_m m_0]$. Therefore on the event $\mathcal{E}_0$, we obtain that $\tilde{R} \le R_B + C_g' p^{-L} + (C_z + 1)\, C_\Xi \kappa_N d_N$, which completes our proof. □

**Proof of Theorem 1**

*Proof.* By inspecting the proof of Theorem 3, one realizes that the proof of Theorem 1 is almost identical to that of Theorem 3 except that the role of Lemma 2 is replaced by the following important lemma under time series structures for different values of $\nu$. More specifically, one only need to show that $\|\hat{\Sigma}_k - \Sigma_k\|_\infty < C_{\ell 1}^{-1}\lambda_{1,N}$ with probability at least $1 - O(p^{-L})$ and the choice of $\lambda_{1,N}$ under time series structures is determined by (result (ii) of the second part in) Lemma 6. Therefore, we omit the proof details.

**Lemma 6.** *Consider the vector linear process defined in (S1.1) that satisfies the decay condition (S1.2). Suppose Conditions 1-3 hold. Recall the number of set from class $k$ is denoted as $N_k = \sum_{i=1}^{N} \mathbb{1}\{\mathcal{Y}_i = k\}$. Then given any positive integer $N_1$ and $N_2$, we have that (i)*

$$\|\hat{\mu}_k - \mu_k\|_\infty \le \begin{cases} C'\sqrt{\frac{\log p}{N_k m_0}} & \text{if } \nu > 1 \\ C'\sqrt{\frac{\log p \log^2 m_0}{N_k m_0}} & \text{if } \nu = 1 \\ C'\sqrt{\frac{\log p}{N_k m_0^{2\nu-1}}} & \text{if } 1/2 < \nu < 1 \end{cases},$$

*and (ii)*

$$\|\hat{\Sigma}_k - \Sigma_k\|_\infty \le \begin{cases} C'\left(\sqrt{\frac{\log p}{N_k m_0}} + \frac{\log p}{N_k m_0}\right) & \text{if } \nu > 1 \\ C'\left(\sqrt{\frac{\log p}{N_k m_0}} + \frac{\log p \log^2 m_0}{N_k m_0}\right) & \text{if } \nu = 1 \\ C'\left(\sqrt{\frac{\log p}{N_k m_0}} + \frac{\log p}{N_k m_0^{2\nu-1}}\right) & \text{if } 3/4 < \nu < 1 \\ C'\left(\sqrt{\frac{\log p \log m_0}{N_k m_0}} + \frac{\log p}{N_k m_0^{1/2}}\right) & \text{if } \nu = 3/4 \\ C'\left(\sqrt{\frac{\log p}{N_k m_0^{4\nu-2}}} + \frac{\log p}{N_k m_0^{2\nu-1}}\right) & \text{if } 1/2 < \nu < 3/4 \end{cases},$$

*for $k = 1, 2$ with probability at least $1 - O(p^{-L})$, where positive constant $C'$ depends on $C_e, c_m, C_{TS}$ and $L$ only.*

*In addition, under the assumption $\log p \le c_0 N$ with some sufficiently small $c_0 > 0$, we*

*have that (i)*

$$\|\hat{\mu}_k - \mu_k\|_\infty \le \begin{cases} C\sqrt{\frac{\log p}{Nm_0}} & \text{if } \nu > 1 \\ C\sqrt{\frac{\log p \log^2 m_0}{Nm_0}} & \text{if } \nu = 1 \\ C\sqrt{\frac{\log p}{Nm_0^{2\nu-1}}} & \text{if } 1/2 < \nu < 1 \end{cases},$$

*and (ii)*

$$\|\hat{\Sigma}_k - \Sigma_k\|_\infty \le \begin{cases} C\sqrt{\frac{\log p}{Nm_0}} & \text{if } \nu > 3/4 \\ C\sqrt{\frac{\log p \log m_0}{Nm_0}} & \text{if } \nu = 3/4 \\ C\sqrt{\frac{\log p}{Nm_0^{4\nu-2}}} & \text{if } 1/2 < \nu < 3/4 \end{cases},$$

*for* $k = 1, 2$ *with probability at least* $1 - O(p^{-L})$*, where positive constant* $C$ *also depends on* $C_\pi$ *besides* $C_e, c_m, C_{TS}$ *and* $L$*.*

□

**Proof of Theorem 2**

*Proof.* By inspecting the proof of Theorem 4, one realizes that the proof of Theorem 2 is almost identical to that of Theorem 4 except that the role of Lemma 3 is replaced by the following important lemma (Lemma 7) under time series structures for different values of $\nu$.

More specifically, the results follow from some algebra (deterministically) on the event that both $\|\tilde{\beta} - \beta\|_\infty \le 6C_{\ell 1}\lambda_{2,N}$ and that $(\beta_1, \beta_2)$ is feasible hold. To this end, Lemma 7 implies that $(\beta_1, \beta_2)$ is feasible with probability at least $1 - O(p^{-L})$. In addition, we show that the choice of $\lambda_{2,N}$ and Lemma 7 together imply that $\|\tilde{\beta} - \beta\|_\infty \le 6C_{\ell 1}\lambda_{2,N}$ with probability

at least $1 - O(p^{-L})$. Indeed, on the event that $(\beta_1, \beta_2)$ is feasible, we have

$$\begin{aligned} \|\Sigma_k\left(\tilde{\beta}_k - \beta_k\right)\|_\infty &\leq \|\hat{\Sigma}_k\left(\tilde{\beta}_k - \beta_k\right)\|_\infty + \|\left(\Sigma_k - \hat{\Sigma}_k\right)\left(\tilde{\beta}_k - \beta_k\right)\|_\infty \\ &\leq \|\hat{\Sigma}_k \beta_k - \hat{\mu}_k\|_\infty + \|\hat{\Sigma}_k \tilde{\beta}_k - \hat{\mu}_k\|_\infty + \|\Sigma_k - \hat{\Sigma}_k\|_\infty \left(\|\beta_k\|_1 + \|\tilde{\beta}_k\|_1\right) \\ &\leq 2\lambda_{2,N} + 2C_\beta C \kappa_\Sigma \leq 3\lambda_{2,N}, \end{aligned}$$

where $\kappa_\Sigma = \sqrt{\frac{\log p}{N m_0}}$ $(\sqrt{\frac{\log p \log m_0}{N m_0}}, \sqrt{\frac{\log p}{N m_0^{4\nu-2}}})$ when $\nu > 3/4$ ($\nu = 3/4$, $1/2 < \nu < 3/4$) respectively. In the above derivation, we have used assumption on $\|\beta_k\|_1$, constraints on estimators, the choice of our $\lambda_{2,N}$ (i.e., $2C_\beta C \kappa_\Sigma \leq \lambda_{2,N}$) and the result (ii) of the second part in Lemma 6. Therefore we further have,

$$\|\tilde{\beta} - \beta\|_\infty \leq \sum_{k=1}^{2} \|\tilde{\beta}_k - \beta_k\|_\infty \leq \sum_{k=1}^{2} \|\Sigma_k^{-1}\|_{\ell_1} \|\Sigma_k\left(\tilde{\beta}_k - \beta_k\right)\|_\infty \leq 6C_{\ell 1}\lambda_{2,N}.$$

Therefore, we complete the proof.

**Lemma 7.** *Consider the vector linear process defined in (S1.1) that satisfies the decay condition (S1.2). Suppose Conditions 1-3 hold. Under the assumptions $\|\beta_k\|_1 \leq C_\beta$, $k = 1, 2$ with some constants $C_\beta > 0$ and $\log p \leq c_0 N$ with some sufficiently small constant $c_0 > 0$, we have that*

$$\|\hat{\Sigma}_k \beta_k - \hat{\mu}_k\|_\infty \leq \begin{cases} C\sqrt{\frac{\log p}{N m_0}} & \text{if } \nu > 1 \\ C\sqrt{\frac{\log p \log^2 m_0}{N m_0}} & \text{if } \nu = 1 \\ C\sqrt{\frac{\log p}{N m_0^{2\nu-1}}} & \text{if } 1/2 < \nu < 1 \end{cases},$$

*for $k = 1, 2$ with probability at least $1 - O(p^{-L})$, where constant $C > 0$ depends on $C_e, c_m, C_\pi, C_\beta, C_\mu, C_{TS}$ and $L$ only.*

□

**Proof of Theorem 3**

*Proof.* By inspecting the proof of Theorem 5, one realizes that the proof of Theorem 3 is very similar to that of Theorem 4. The major differences are that $\beta_0$ is replaced by $\beta_{0,TS}$ and that the role of Lemma 5 is replaced by Lemma 8 under time series structures for different values of $\nu$, which is provided at the end of this proof.

We only highlight the differences from the proof of Theorem 3 below briefly.

We still define $\tilde{Z}_i = \log(\hat{\pi}_1/\hat{\pi}_2)/M_i + \bar{X}_i^T\tilde{\beta} + \bar{X}_i^T\tilde{\nabla}\bar{X}_i/2 + \mathrm{tr}(\tilde{\nabla}S_i)/2$, which is used to approximate $Z_i = \log(\pi_1/\pi_2)/M_i + \bar{X}_i^T\beta + \bar{X}_i^T\nabla\bar{X}_i/2 + \mathrm{tr}(\nabla S_i)/2$. Note that under the general time series structures, $\beta_{0,TS}$ is the population minimizer of the loss function. Thus, we can still obtain the inequality similar to (S2.26), i.e.,

$$\begin{aligned}\ell_0(\tilde{\beta}_0, \tilde{Z}) &\leq \ell_0(\beta_{0,TS}, \tilde{Z}) + E_{\beta_{0,TS}} - E_{\tilde{\beta}_0} \\ &\leq \ell_0(\beta_{0,TS}, \tilde{Z}) + m_0 R_1 \left|\tilde{\beta}_0 - \beta_{0,TS}\right|, \qquad \text{(S2.34)}\end{aligned}$$

where $R_1 = |\frac{1}{Nm_0}\Sigma_{i=1}^N(\mathcal{Y}_i - \mathbb{E}(\mathcal{Y}_i|\mathcal{X}_i))M_i| \leq C_r\sqrt{(\log p)/N}$ with probability at least $1-O(p^{-L})$ by Hoeffding's inequality. Again, this statement is valid conditioning on any realization of $\{\mathcal{X}_i\}_{i=1}^N$ and thus is also valid unconditionally.

In addition, applying Lemma 4 to $\ell_0(\theta_0, \tilde{Z})$ at point $\beta_{0,TS}$ and by Condition 2, we still have (S2.27) with $\beta_0$ being replaced by $\beta_{0,TS}$, i.e.,

$$\begin{aligned}&\ell_0(\tilde{\beta}_0, \tilde{Z}) - \ell_0(\beta_{0,TS}, \tilde{Z}) \qquad \text{(S2.35)}\\ \geq\; &\ell_0'(\beta_{0,TS}, \tilde{Z})(\tilde{\beta}_0 - \beta_{0,TS}) + \frac{\ell_0''(\beta_{0,TS}, \tilde{Z})}{C_m^2 m_0^2}(e^{-C_m m_0|\tilde{\beta}_0 - \beta_{0,TS}|} + C_m m_0\left|\tilde{\beta}_0 - \beta_{0,TS}\right| - 1).\end{aligned}$$

We next bound $\ell_0'(\beta_{0,TS}, \tilde{Z})$ from above and bound $\ell_0''(\beta_{0,TS}, \tilde{Z})$ from below.

By applying Lemma 8 and our assumption, we have that with probability at least $1 - O(p^{-L})$, $m_0 \max_i |\tilde{Z}_i - Z_i| := R_2$ is sufficiently small. Therefore, with the fact that $\ell_0'(\beta_{0,TS}, Z) =$

0 where $\ell_0'(\beta_{0,TS}, Z)$ is obtained by replacing $\tilde{Z}_i$ by $Z_i$ in $\ell_0'(\beta_{0,TS}, \tilde{Z})$, $i = 1, \ldots, N$, we can still obtain an upper bound $|\ell_0'(\beta_{0,TS}, \tilde{Z})|$ similar to (S2.29), i.e.,

$$\begin{aligned} \left|\ell_0'(\beta_{0,TS}, \tilde{Z})\right| &= \left|\frac{1}{N}\Sigma_{i=1}^N\left(\frac{M_i\exp(M_i(\beta_{0,TS}+\tilde{Z}_i))}{1+\exp(M_i(\beta_{0,TS}+\tilde{Z}_i))} - \frac{M_i\exp(M_i(\beta_{0,TS}+Z_i))}{1+\exp(M_i(\beta_{0,TS}+Z_i))}\right)\right| \\ &\leq C_m^2 m_0 R_2, \end{aligned} \tag{S2.36}$$

Moreover, by Condition 1, we have that the expectation of the i.i.d. bounded random variable $\frac{\exp(M_i(\beta_0+Z_i))}{(1+\exp(M_i(\beta_0+Z_i)))^2}$, $i = 1, \ldots, N$, is bounded away from $C_{\log}$. Following a similar argument, we are able to obtain a similar result to (S2.30), i.e., with probability at least $1 - O(p^{-L})$,

$$\begin{aligned} \ell_0''(\beta_{0,TS}, \tilde{Z}) &= \frac{1}{N}\Sigma_{i=1}^N M_i^2\left(\frac{\exp\left(M_i(\beta_{0,TS}+\tilde{Z}_i)\right)}{1+\exp\left(M_i(\beta_{0,TS}+\tilde{Z}_i)\right)}\right)\left(\frac{1}{1+\exp\left(M_i(\beta_{0,TS}+\tilde{Z}_i)\right)}\right) \\ &\geq C_{low} m_0^2. \end{aligned} \tag{S2.37}$$

In the end, plugging (S2.34), (S2.36) and (S2.37) into (S2.35) and applying the union bound argument, we obtain that with probability $1 - O(p^{-L})$,

$$C_{low}C_m^{-2}(e^{-C_m m_0\left|\tilde{\beta}_0-\beta_{0,TS}\right|}+C_m m_0\left|\tilde{\beta}_0-\beta_{0,TS}\right|-1) \leq m_{0,TS}\left(C_m^2 R_2 + R_1\right)\left|\tilde{\beta}_0 - \beta_0\right|. \tag{S2.38}$$

Then following a similar deterministic argument, we obtain that with probability $1-O(p^{-L})$,

$$\left|\tilde{\beta}_0 - \beta_{0,TS}\right| \leq 2C_{low}^{-1} m_0^{-1}\left(C_m^2 R_2 + R_1\right),$$

which further completes our proof, together with Lemma 8 and the bound of $R_1$,

$$\left|\tilde{\beta}_0 - \beta_{0,TS}\right| \leq C_\delta\left((1+U_\beta)\|\tilde{\beta}-\beta\|_1 + (1+U_\nabla)\|\tilde{\nabla}-\nabla\|_1 + \max_{k=1,2}\frac{|\pi_k - \hat{\pi}_k|}{m_0} + \sqrt{\frac{\log p}{Nm_0^2}}\right).$$

**Lemma 8.** *Under the assumptions of Theorem 3, there exists some constant $C_z > 0$ depending on $c_m, C_m, C_\pi, C_\mu, C_{TS}$ and $C_e$ such that with probability at least $1-O(p^{-L})$ we have*

*uniformly for all* $i = 1, \ldots, N$

$$\begin{aligned}\left|\tilde{Z}_i - Z_i\right| &\leq \frac{1}{M_i}\left|\log\left(\frac{\hat{\pi}_1\pi_2}{\hat{\pi}_2\pi_1}\right)\right| + \left|\bar{X}_i^T\left(\tilde{\beta}-\beta\right)\right| + \frac{1}{M_i}\left|\sum_{j=1}^{M_i} X_{ij}^T\left(\tilde{\nabla}-\nabla\right)X_{ij}/2\right| \\ &\leq C_z\left((1+U_\beta)\|\tilde{\beta}-\beta\|_1 + (1+U_\nabla)\|\tilde{\nabla}-\nabla\|_1 + \max_{k=1,2}\frac{|\pi_k - \hat{\pi}_k|}{m_0}\right), \quad \text{(S2.39)}\end{aligned}$$

*where* $U_\beta$ *satisfies*

$$U_\beta = \begin{cases} \sqrt{\frac{\log p}{m_0}} & \text{if } \nu > 1 \\ \sqrt{\frac{\log p \log^2 m_0}{m_0}} & \text{if } \nu = 1 \\ \sqrt{\frac{\log p}{m_0^{2\nu-1}}} & \text{if } 1/2 < \nu < 1 \end{cases},$$

*and* $U_\nabla$ *satisfies*

$$U_\nabla = \begin{cases} \frac{\log p}{m_0} & \text{if } \nu > 1 \\ \frac{\log p \log^2 m_0}{m_0} & \text{if } \nu = 1 \\ \frac{\log p}{m_0^{2\nu-1}} & \text{if } 1/2 < \nu < 1 \end{cases}.$$

*Indeed, the conclusion (S2.39) is valid with the same probability* $1 - O(p^{-L})$ *conditioning on any realization of* $\{\mathcal{Y}_i\}_{i=1}^N$ *and* $\{M_i\}_{i=1}^N$.

□

**Proof of Theorem 4**

*Proof.* By inspecting the proof of Theorem 6, one realizes that the proof of Theorem 4 is almost identical to that of Theorem 6 with $\phi_B$, $\beta_0$, $\Xi_N$, $\kappa_N$, $F_{k,m}$ and $R_B$ being replaced by their counterparts $\phi_{B,TS}$, $\beta_{0,TS}$, $\Xi_{N,TS}$, $\kappa_{N,TS}$, $F_{k,m,TS}$ and $R_{B,TS}$ under the time series structure respectively. Therefore, we omit the proof details. □

## S3. Proofs of Supporting Lemmas

### Proof of Lemma 1

*Proof.* Recall $n_1 = \sum_{i=1}^N M_i \mathbb{1}\{\mathcal{Y}_i = 1\}$ with $\mathbb{1}\{\mathcal{Y}_i = 1\}$ i.i.d. Bernoulli with probability $\pi_1 \in [C_\pi, 1 - C_\pi]$ and $M_i \in [c_m m_0, C_m m_0]$ with probability 1. Hoeffding's inequality (e.g. Vershynin, 2012, Proposition 5.10) implies that there exists some constant $C'$ depending on $C_\pi$ and $L$ only such that (iv) holds, i.e. $|\pi_1 - \hat{\pi}_1| \le C'\sqrt{\frac{\log p}{N}}$ with probability at least $1 - p^{-L}$. Consequently, $n_1 \ge cNm_0$ for some constant $c$ depending on $c_m, C_\pi$ and $L$ with probability at least $1 - p^{-L}$ given $\log p \le c_0 N$ and Condition 3. Similar results apply to $\hat{\pi}_2$ and $n_2$. From now on, we condition on the above event and only need to show (i)-(iii) hold with probability at least $1 - p^{-L}$.

Since $\Sigma_k^{-1/2}(\hat{\mu}_k - \mu_k) \sim N(0, \frac{1}{n_k} I_p)$, the tail probability of Chi-squared distribution (Laurent and Massart, 2000, e.g.) implies that for any $0 < t < 1$, $\mathrm{pr}(|\|\sqrt{n_k}\Sigma_k^{-1/2}(\hat{\mu}_k - \mu_k)\|^2/p - 1| \ge t) \le 2\exp(pt^2/8)$. Hence, by picking a small $t$ (e.g. $t = 0.1$) as well as Condition 1 and $n_k > cNm_0$, we obtain the result (ii) holds with probability at least $1 - O(p^{-L})$.

In addition, it follows from the Davidson-Szarek bound (e.g. Davidson and Szarek, 2001, Theorem II.7) that for each $k$, there exists some constant $C > 0$ depending on $C_e, L$ such that $\|\Sigma_k - \hat{\Sigma}_k\|_{\ell_2} < C\sqrt{p/(Nm_0)}$ with probability at least $1 - 2p^{-L}$, given Condition 1 and the fact $p < c_0 N m_0$ with a sufficiently small $c_0$. Here $\|\cdot\|_{\ell_2}$ denotes the matrix spectral norm. Consequently, the assumption $p < c_0 N m_0$ and Condition 1, together with a union bound argument, implies the result (i). Result (iv) also follows, noting that $\|\cdot\|_F \le \sqrt{p}\|\cdot\|_{\ell_2}$. $\square$

**Proof of Lemma 2**

*Proof.* Recall that $n_k = \sum_{i=1}^N M_i \mathbb{1}\{\mathcal{Y}_i = k\}$ denote the total sample size for Class $k = 1, 2$. From now on, we condition on $n_1$ and $n_2$. Write $X_{ij} = \mathbb{E}X_{ij} + U_{ij}$, where $U_{ij} \sim N(0, \Sigma_{\mathcal{Y}_i})$. Then we have $\hat{\Sigma}_k = (\frac{1}{n_k}\sum_{(i,j):\mathcal{Y}_i=k} U_{ij}U_{ij}^T) - (\mu_k - \hat{\mu}_k)(\mu_k - \hat{\mu}_k)^T$. Since $\hat{\mu}_k - \mu_k \sim N(0, \frac{1}{n_k}\Sigma_k)$, tail probability of normal distribution with union bound implies that for any $L > 0$, there exists some constant $C_1 > 0$ depending on $L$ only such that for $k = 1, 2$,

$$\mathrm{pr}(\|\hat{\mu}_k - \mu_k\|_\infty \geq C_1\sqrt{\frac{(\max_j \sigma_{k,jj})\log p}{n_k}}) \leq p^{-L}. \tag{S3.40}$$

Moreover, since $\mathbb{E}\frac{1}{n_k}\sum_{(i,j):\mathcal{Y}_i=k} U_{ij}U_{ij}^T = \Sigma_k$ and each entry of $U_{ij}U_{ij}^T$ is sub-exponentially distributed, Bernstein's inequality (e.g. Vershynin, 2012, Proposition 5.16) with union bound implies that there exists some constant $C_2 > 0$ depending on $L$ such that

$$\mathrm{pr}(\|\frac{1}{n_k}\sum_{(i,j):\mathcal{Y}_i=k} U_{ij}U_{ij}^T - \Sigma_k\|_\infty \geq C_2 \max_j \sigma_{k,jj}(\sqrt{\frac{\log p}{n_k}} + \frac{\log p}{n_k})) \leq p^{-L}. \tag{S3.41}$$

Combining (S3.40) and (S3.41) and the fact that $M_i \in [c_m m_0, C_m m_0]$, we have obtained both results (i) and (ii) of the first part of Lemma 2 with probability at least $1 - 4p^{-L}$, where the constant $C' > 0$ depends on $c_m, C_e$ and $L$ only.

We move to the second part of Lemma 2. Note the distribution of each $X_{ij}$ is independent of $N_k$ and $n_k$. We follow the same argument on bounding $n_1$ and $n_2$ as that at the beginning of the proof of Lemma 1. In particular, given $\log p \leq c_0 N$, we have $\mathrm{pr}(n_k \geq cNm_0) = 1 - p^{-L}$ for $k = 1, 2$ and some constant $c > 0$. Then both results (i) and (ii) of the second part of Lemma 2 immediately follow from the first part of Lemma 2 and a union bound argument. □

**Proof of Lemma 3**

*Proof.* We follow the same argument on bounding $n_1$ and $n_2$ as that at the beginning of the proof of Lemma 1. In particular, given $\log p \leq c_0 N$, we have $\text{pr}(n_k \geq cNm_0) = 1 - p^{-L}$ for $k = 1, 2$ and some constant $c > 0$.

Write $X_{ij} = \mathbb{E}X_{ij} + U_{ij}$, where $U_{ij} \sim N(0, \Sigma_{\mathcal{Y}_i})$. We have $\hat{\Sigma}_k = (\frac{1}{n_k}\sum_{(i,j):\mathcal{Y}_i = k} U_{ij}U_{ij}^T) - (\mu_k - \hat{\mu}_k)(\mu_k - \hat{\mu}_k)^T$. Result (i) of Lemma 2 implies that there exists some constant $C_1 > 0$ such that

$$\text{pr}(\|\hat{\mu}_k - \mu_k\|_\infty \geq C_1\sqrt{\frac{\log p}{Nm_0}}) = O(p^{-L}). \tag{S3.42}$$

According to our assumptions, we have $\|\Sigma_k^{-1}\mu_k\| \leq \lambda_{\min}^{-1}(\Sigma_k)\|\mu_k\| \leq C_e C_\mu$. We condition on $n_1$ and $n_2$. Then the normality of $\hat{\mu}_k - \mu_k \sim N(0, \Sigma_k/n_k)$ yields that for $k = 1, 2$ and some constant $C''$ depending on $L$ only, we have $\left|(\mu_k - \hat{\mu}_k)^T\Sigma_k^{-1}\mu_k\right| \geq C''\lambda_{\max}(\Sigma_k)C_e C_\mu\sqrt{\frac{\log p}{n_k}}$ with probability at most $p^{-L}$. Taking union bound with the event $n_k \geq cNm_0$, we obtain that there exists some constant $C_2' > 0$ such that

$$\text{pr}(\left|(\mu_k - \hat{\mu}_k)^T\Sigma_k^{-1}\mu_k\right| \geq C_2'\sqrt{\frac{\log p}{Nm_0}}) \leq 2p^{-L}. \tag{S3.43}$$

Therefore, equations (S3.42)-(S3.43) imply that here exists some constant $C_2 > 0$ such that with probability $1 - O(p^{-L})$,

$$\|(\mu_k - \hat{\mu}_k)(\mu_k - \hat{\mu}_k)^T\beta_k\|_\infty < C_2\frac{\log p}{Nm_0}. \tag{S3.44}$$

By our choice of $\lambda_{2,N}$, we have that $\lambda_{2,N}/2 > (C_1 + C_2 + C_2')\sqrt{(\log p)/(Nm_0)}$. Consequently, given equations (S3.42)-(S3.44), decomposition of $\Sigma_k$ and $\log p = o(N)$, to conclude $(\beta_1, \beta_2)$ is feasible, i.e. $\left\|\hat{\Sigma}_k\beta_k - \hat{\mu}_k\right\|_\infty < \lambda_{2,N}$, $k = 1, 2$, we only need to show with probability

$1 - O(p^{-L})$ that

$$\|(\frac{1}{n_k}\sum_{(i,j):\mathcal{Y}_i=k} U_{ij}U_{ij}^T)\Sigma_k^{-1}\mu_k - \mu_k\|_\infty < \frac{1}{2}\lambda_{2,N}. \tag{S3.45}$$

Note that the $r$th coordinate is $\frac{1}{n_k}\sum_{(i,j):\mathcal{Y}_i=k}\left(U_{ij,r}U_{ij}^T\Sigma_k^{-1}\mu_k - \mu_{k,r}\right)$, the sum of i.i.d. centered sub-exponential variable since each summand is the product of two normal variables $U_{i,j}$ and $U_i^T\Sigma_k^{-1}\mu_k$. Moreover, the sub-exponential variable has constant parameter since $U_{ij}^T\Sigma_k^{-1}\mu_k$ and $U_{ij,r}$ have bounded variance. Thus Bernstein's inequality (e.g. Vershynin, 2012, Proposition 5.16) with union bound over all coordinates and the event $n_k \geq cNm_0$ implies that there exists some constant $C_3 > 0$ such that (we also used that $\log p \leq c_0 N$ when applying the Bernstein's inequality)

$$\mathrm{pr}(\|(\frac{1}{n_k}\sum_{(i,j):\mathcal{Y}_i=k} U_{ij}U_{ij}^T)\Sigma_k^{-1}\mu_k - \mu_k\|_\infty > C_3\sqrt{\frac{\log p}{Nm_0}}) \leq 2p^{-L}. \tag{S3.46}$$

By picking a large constant $C'$ in our choice of $\lambda_{2,N}$, we obtain $\lambda_{2,N}/2 > C_3\sqrt{(\log p)/(Nm_0)}$, which completes the proof of (S3.45). □

### Proof of Lemma 5

*Proof.* It is sufficient to show that for any realization of $\{\mathcal{Y}_i\}_{i=1}^N$ and $\{M_i\}_{i=1}^N$, equation (S2.28) is valid for each $i$ with probability at least $1 - O(p^{-L-1})$. Indeed, this fact, together with the union bound argument and $p \geq N$ implies the desired result. The first inequality of (S2.28) follows from the definitions of $\tilde{Z}_i$ and $Z_i$ directly. We show the second inequality holds in the remaining of proof with probability at least $1 - O(p^{-L-1})$ for the fixed $i$. Without loss of generality, we assume $\mathcal{Y}_i = 1$ and $M_i = m_0 c_m$.

Recall that the initial estimators satisfy $\max_{k=1,2}|\pi_k - \hat{\pi}_k| \leq C_p$ with a sufficiently small constant $C_p$. Consequently, we have that $\hat{\pi}_1, \hat{\pi}_2 \in [C_\pi/2, 1 - C_\pi/2]$ by Condition 3, which

further yields $\frac{1}{m_0 c_m}\left|\log\left(\frac{\hat{\pi}_1\pi_2}{\hat{\pi}_2\pi_1}\right)\right| \le C_{z1}\max_{k=1,2}|\pi_k - \hat{\pi}_k|/m_0$ with some universal constant $C_{z1}$ depending on $c_m$ and $C_\pi$ only by the boundedness of $\hat{\pi}_1/\hat{\pi}_2$.

To deal with the term $|\bar{X}_i^T(\tilde{\beta}-\beta)|$, we note that $\bar{X}_i \sim N(\mu_1, \Sigma_1/(m_0 c_m))$, which implies that $|\bar{X}_i^T(\tilde{\beta}-\beta)| \le \|\tilde{\beta}-\beta\|\cdot\|\mu_1\| + \|\tilde{\beta}-\beta\|\left(C_e/(m_0 c_m)\right)^{1/2}|D|$, where $D \sim N(0,1)$. According to the tail probability of standard normal distribution, we obtain that with probability at least $1-O(p^{-L-1})$, that $|D| \le C_z'\sqrt{\log p}$ where $C_z'$ only depends on $L$. This fact, together with the assumption $\|\mu_1\| \le C_\mu$ further implies that $|\bar{X}_i^T(\tilde{\beta}-\beta)| \le C_{z2}\|\tilde{\beta}-\beta\|(1+\sqrt{(\log p)/m_0})$ with probability $1-O(p^{-L-1})$, where $C_{z2} = ((C_e/c_m)^{1/2}C_z' + C_\mu)$.

Finally, we provide an upper bound for $\frac{1}{M_i}\left|\sum_{j=1}^{M_i} X_{ij}^T(\tilde{\nabla}-\nabla)X_{ij}/2\right|$. Since $X_{i1},\dots,X_{iM_i}$ are i.i.d. copies of $N(\mu_1,\Sigma_1)$, we naturally decompose it into three terms as follows with $U_{ij} := X_{ij}-\mu_1 \sim N(0,\Sigma_1)$

$$\begin{aligned}&\frac{1}{M_i}\left|\sum_{j=1}^{M_i} X_{ij}^T\left(\tilde{\nabla}-\nabla\right)X_{ij}/2\right|\\ \le\ &\frac{1}{M_i}\left|\sum_{j=1}^{M_i} U_{ij}^T\left(\tilde{\nabla}-\nabla\right)U_{ij}/2\right| + \left|\mu_1^T\left(\tilde{\nabla}-\nabla\right)\mu_1/2\right| + \frac{1}{M_i}\left|\sum_{j=1}^{M_i}\mu_1^T\left(\tilde{\nabla}-\nabla\right)U_{ij}\right|\end{aligned} \tag{S3.47}$$

We deal with these three terms individually. First of all, $|\mu_1^T(\tilde{\nabla}-\nabla)\mu_1/2| \le C_\mu^2\|\tilde{\nabla}-\nabla\|_1/2$ by the assumption $\|\mu_1\| \le C_\mu$. Second, the term $(\sum_{j=1}^{M_i}\mu_1^T(\tilde{\nabla}-\nabla)U_{ij})/M_i$ follows a distribution of $N(0, \mu_1^T(\tilde{\nabla}-\nabla)\Sigma_1(\tilde{\nabla}-\nabla)\mu_1/(m_0 c_m))$, which yields that with probability at least $1-O(p^{-L-1})$ that

$$\begin{aligned}\frac{1}{M_i}\left|\sum_{j=1}^{M_i}\mu_1^T\left(\tilde{\nabla}-\nabla\right)U_{ij}\right| &\le \left(\mu_1^T\left(\tilde{\nabla}-\nabla\right)\Sigma_1\left(\tilde{\nabla}-\nabla\right)\mu_1/(m_0 c_m)\right)^{1/2} C_z''\sqrt{\log p}\\ &\le C_\mu C_z'\left(C_e/c_m\right)^{1/2}\|\tilde{\nabla}-\nabla\|_1\sqrt{\frac{\log p}{m_0}},\end{aligned}$$

where we have used tail probability of standard normal distribution and the last inequality

follows from Condition 1. Third, by Hölder's inequality, we have

$$\begin{aligned}\frac{1}{M_i}\left|\sum_{j=1}^{M_i} U_{ij}^T\left(\tilde{\nabla}-\nabla\right)U_{ij}/2\right| &= \left|\mathrm{tr}(\left(\tilde{\nabla}-\nabla\right)\sum_{j=1}^{M_i} U_{ij}^T U_{ij}/M_i)/2\right| \\ &\leq \frac{1}{2}\left\|\tilde{\nabla}-\nabla\right\|_1\left\|\sum_{j=1}^{M_i} U_{ij}^T U_{ij}/M_i\right\|_\infty .\end{aligned}$$

Since each entry of $\sum_{j=1}^{M_i} U_{ij}^T U_{ij}/M_i - \Sigma_1$ is the sum of centered sub-exponential variable with bounded parameter. The Bernstein's inequality (e.g. Vershynin, 2012, Proposition 5.16) with union bound over all $p^2$ entries implies that there exists some constant $C_z'' > 0$ depending on $L$ and $C_e$ only such that $\left\|\sum_{j=1}^{M_i} U_{ij}^T U_{ij}/M_i - \Sigma_1\right\|_\infty \leq C_z''(\sqrt{\frac{\log p}{c_m m_0}} + \frac{\log p}{c_m m_0})$ with probability at least $1 - O(p^{-L-1})$. Therefore, we obtain that with probability $1 - O(p^{-L-1})$,

$$\frac{1}{M_i}\left|\sum_{j=1}^{M_i} U_{ij}^T\left(\tilde{\nabla}-\nabla\right)U_{ij}/2\right| \leq (C_z''(\sqrt{\frac{\log p}{c_m m_0}} + \frac{\log p}{c_m m_0}) + C_e)\|\tilde{\nabla}-\nabla\|_1/2,$$

where we have used $\|\Sigma_1\|_\infty \leq C_e$ by Condition 1. Combining the upper bounds of three terms above, we finally obtain that with probability $1 - O(p^{-L-1})$,

$$\begin{aligned}\frac{1}{M_i}\left|\sum_{j=1}^{M_i} X_{ij}^T\left(\tilde{\nabla}-\nabla\right)X_{ij}/2\right| &\leq C_{z3}'(\sqrt{\frac{\log p}{m_0}} + \frac{\log p}{m_0} + 1)\|\tilde{\nabla}-\nabla\|_1 \\ &\leq C_{z3}(\frac{\log p}{m_0} + 1)\|\tilde{\nabla}-\nabla\|_1,\end{aligned}$$

where constant $C_{z3}' = C_\mu^2/2 + C_\mu C_z' \left(C_e/c_m\right)^{1/2} + (C_e + C_z''/\sqrt{c_m} + C_z''/c_m)/2$ and $C_{z3} = 2C_{z3}'$.

To complete our proof, we combine all bounds for $\frac{1}{m_0 c_m}\left|\log\left(\frac{\hat{\pi}_1\pi_2}{\hat{\pi}_2\pi_1}\right)\right|$, $|\bar{X}_i^T(\tilde{\beta}-\beta)|$ and $\frac{1}{M_i}|\sum_{j=1}^{M_i} X_{ij}^T(\tilde{\nabla}-\nabla)X_{ij}/2|$ with $C_z = C_{z1} + C_{z2} + C_{z3}$. □

**Proof of Lemma 6**

*Proof.* We show the first part of Lemma 6 in this proof. The second part of Lemma 6 immediately follows from the first part, that $\log p \leq c_0 N$, and the fact that $\mathrm{pr}(n_k \geq cNm_0) =$

$1 - p^{-L}$ for $k = 1, 2$ and some constant $c > 0$, which is obtained from the argument at the beginning of the proof of Lemma 1.

In this proof, we need the following technical result, which is a direct consequence of Lemma VI.1 in Chen et al. (2016).

**Lemma 9** (Chen et al. (2016)). *Let $\nu > 1/2$ and $(a_t)_{t\in\mathbb{Z}}$ be a real sequence such that $a_t \le C_{TS}(1+t)^{-\nu}$ for $t \ge 0$ and $a_t = 0$ if $t < 0$. Let $\gamma_l = \sum_{t=0}^{\infty} |a_t a_{t+l}|$. Then (i) $\gamma_l = O(l^{-\nu})$ $(O(l^{-1}\log l)$ and $O(l^{1-2\nu}))$ and $\sum_{k=0}^{l} \gamma_k = O(1)$ $(O(\log^2 l)$ and $O(l^{2-2\nu}))$ hold for $\nu > 1$ ($\nu = 1$ and $1/2 < \nu < 1$ respectively); (ii) $\sum_{k=0}^{l} \gamma_k^2 = O(1)$ $(O(\log l)$ and $O(l^{3-4\nu}))$ hold for $\nu > 3/4$ ($\nu = 3/4$ and $1/2 < \nu < 3/4$ respectively).*

Without loss of generality, we assume that the first $N_1$ sets are from Class 1 (i.e., $\mathcal{Y}_i = 1$ for $i = 1, ..., N_1$) and only prove results (i)-(ii) for Class 1. We first show result (i), i.e., bound the term $\|\mu_1 - \hat{\mu}_1\|_\infty$. In the following, we bound each entry of $\mu_1 - \hat{\mu}_1$ and then take a union bound argument to finish the proof. To bound the $l$th entry ($l = 1, ..., p$), i.e., $|\mu_{1l} - \hat{\mu}_{1l}|$, we collect the $l$th entry $X_{ij,l}$ of each observation $X_{ij}$, $i = 1, ..., N_1$, $j = 1, ..., M_i$ and observe that its centered version can be denoted according to the vector linear process (S1.1) as

$$(X_{1M_1,l}, ..., X_{11,l}; X_{2M_2,l}, ..., X_{21,l}; ...; X_{N_1 M_{N_1},l}, ..., X_{N_1 1,l})^T - (\mu_{1l}, ..., \mu_{1l})^T = \mathbf{A}^{(l)} \boldsymbol{\xi}, \quad \text{(S3.48)}$$

where $\boldsymbol{\xi} = (\xi_{1M_1}, \xi_{1(M_1-1)} ...; \xi_{2M_2}, \xi_{2(M_2-1)} ...; ...; \xi_{N_1 M_{N_1}}, \xi_{N_1(M_{N1}-1)} ...)^T$ with i.i.d. $N(0, 1)$ en-

tries, and $\mathbf{A}^{(l)}$ is a block diagonal matrix,

$$\mathbf{A}^{(l)} = \begin{bmatrix} \mathbf{A}^{(l),1} & 0 & 0 & 0 \\ 0 & \mathbf{A}^{(l),2} & 0 & 0 \\ \vdots & \vdots & \ddots & \\ 0 & 0 & 0 & \mathbf{A}^{(l),N_1} \end{bmatrix},$$

in which the $i$ the block ($i = 1, ..., N_1$) $\mathbf{A}^{(l),i}$ has the following form

$$\mathbf{A}^{(l),i} = \begin{bmatrix} A_{10,l\cdot} & A_{11,l\cdot} & A_{12,l\cdot} & \dots & A_{1(M_i-1),l\cdot} & A_{1M_i,l\cdot} & \dots \\ 0 & A_{10,l\cdot} & A_{11,l\cdot} & \dots & A_{1(M_i-2),l\cdot} & A_{1(M_i-1),l\cdot} & \dots \\ 0 & 0 & A_{10,l\cdot} & \dots & A_{1(M_i-3),l\cdot} & A_{1(M_i-2),l\cdot} & \dots \\ \vdots & \vdots & \vdots & \ddots & \vdots & \vdots & \vdots \\ 0 & 0 & 0 & \dots & A_{10,l\cdot} & A_{11,l\cdot} & \dots \end{bmatrix}.$$

In the above representation, $A_{1t,l\cdot}$ denotes the $l$th row of the coefficient matrix $A_{1t}$ defined in our vector linear process (S1.1). Given (S3.48), one immediately obtains that

$$\mu_1 - \hat{\mu}_1 \sim N\left(0, \mathbf{1}^T \mathbf{A}^{(l)} \left(\mathbf{A}^{(l)}\right)^T \mathbf{1}/n_1^2\right), \tag{S3.49}$$

where $n_1 = \sum_{i=1}^{N_1} M_i$ denote the total sample size for Class 1, and $\mathbf{1}$ denotes the $n_1$-dimensional vector with each entry being 1.

It remains to bound the variance in (S3.49) for different value of $\nu > 1/2$. To this end, we note that

$$\mathbf{1}^T \mathbf{A}^{(l)} \left(\mathbf{A}^{(l)}\right)^T \mathbf{1} = \sum_{i=1}^{N_1} \mathbf{1}^T \mathbf{A}^{(l),i} \left(\mathbf{A}^{(l),i}\right)^T \mathbf{1} := \sum_{i=1}^{N_1} \mathbf{1}^T \Gamma^{(l),i} \mathbf{1},$$

where we set $\Gamma^{(l),i} = \mathbf{A}^{(l),i} \left(\mathbf{A}^{(l),i}\right)^T$ and $\mathbf{1}$ in the $i$th summand denotes the $M_i$-dimensional vector with each entry being 1 respectively. Due to the time series structure, the matrix

$\Gamma^{(l),i}$ is a $M_i$-dimensional Toeplitz matrix with elements $(\gamma_j^l)_{j=0}^{M_i-1}$, where

$$\begin{aligned} |\gamma_j^l| &= \left|\sum_{t=0}^{\infty} A_{1t,l\cdot}\left(A_{1(t+j),l\cdot}\right)^T\right| \\ &\leq \sum_{t=0}^{\infty}\left(\left(\sum_{k=1}^{p} a_{1t,lk}^2\right)^{1/2}\left(\sum_{k=1}^{p} a_{1(t+j),lk}^2\right)^{1/2}\right) \\ &\leq C\zeta_j, \end{aligned} \tag{S3.50}$$

where $C > 0$ is some constant, $\zeta_j = j^{-\nu}$ ($j^{-1}\log j$ and $j^{1-2\nu}$) for $\nu > 1$ ($\nu = 1$ and $1/2 < \nu < 1$ respectively). The first inequality above follows from Cauchy-Schwarz inequality and the second inequality is due to the decay condition of the coefficient matrix in (S1.2) and Lemma 9 (i). Consequently, we can bound the variance as follows, noting that $n_1 > c_m N_1 m_0$ by Condition 3,

$$\begin{aligned} \frac{\mathbf{1}^T\mathbf{A}^{(l)}\left(\mathbf{A}^{(l)}\right)^T\mathbf{1}}{n_1^2} &\leq \frac{\sum_{i=1}^{N_1} M_i\sum_{j=0}^{M_i-1}\zeta_j}{(c_m N_1 m_0)^2} \\ \leq \quad \frac{C_m N_1 m_0\sum_{j=0}^{C_m m_0-1}\zeta_j}{(c_m N_1 m_0)^2} &\leq \begin{cases} C\frac{1}{N_1 m_0} & \text{if } \nu > 1 \\ C\frac{\log^2 m_0}{N_1 m_0} & \text{if } \nu = 1 \\ C\frac{1}{N_1 m_0^{2\nu-1}} & \text{if } 1/2 < \nu < 1 \end{cases}, \end{aligned}$$

where the last inequality follows from Lemma 9 (i). In the end, the result (i) of the first part immediately follows from the above variance bound and the the tail probability of normal distribution with a union bound argument.

Now we turn to the result (ii). In the following, we bound each entry of $\Sigma_1 - \hat{\Sigma}_1$ and then take a union bound argument to finish the proof. To bound the $lk$th entry ($l, k = 1, ..., p$), i.e., $|\sigma_{1,lk} - \hat{\sigma}_{1,lk}|$, we note that

$$\sigma_{1,lk} - \hat{\sigma}_{1,lk} = \frac{1}{n_1}\left(\boldsymbol{\xi}^T\left(\mathbf{A}^{(l)}\right)^T\mathbf{A}^{(k)}\boldsymbol{\xi} - \mathbb{E}\boldsymbol{\xi}^T\left(\mathbf{A}^{(l)}\right)^T\mathbf{A}^{(k)}\boldsymbol{\xi}\right) - (\mu_{1l} - \hat{\mu}_{1l})(\mu_{1k} - \hat{\mu}_{1k}) := T_1 + T_2, \tag{S3.51}$$

where the second term can be bounded with probability at least $1 - O(p^{-(L+2)})$ using the result (i) shown above, that is,

$$|T_2| \le \begin{cases} C\frac{\log p}{N_1 m_0} & \text{if } \nu > 1 \\ C\frac{\log p \log^2 m_0}{N_1 m_0} & \text{if } \nu = 1 \\ C\frac{\log p}{N_1 m_0^{2\nu-1}} & \text{if } 1/2 < \nu < 1 \end{cases}.$$

It remains to bound the first term $|T_1|$. To this end, we apply the Hanson-Wright inequality (e.g. Rudelson and Vershynin, 2013, Theorem 1.1) since $\boldsymbol{\xi}$ contains i.i.d $N(0,1)$ entries. Note that by Condition 3, we have $c_m m_0 \le M_i \le C_m m_0$. Therefore,

$$\begin{aligned} & \text{pr}\left(|T_1| \ge x\right) \qquad \text{(S3.52)} \\ \le\ & 2\exp\left(-C\min\left\{\|\left(\mathbf{A}^{(l)}\right)^T\mathbf{A}^{(k)}\|)_F^{-2}x^2N_1^2m_0^2, \lambda_{\max}^{-1}\left(\left(\mathbf{A}^{(l)}\right)^T\mathbf{A}^{(k)}\right)xN_1m_0\right\}\right), \end{aligned}$$

where $\lambda_{\max}(\cdot)$ denotes the largest singular value. In what follows, we bound $\|\left(\mathbf{A}^{(l)}\right)^T\mathbf{A}^{(k)}\|_F^2$ and $\lambda_{\max}\left(\left(\mathbf{A}^{(l)}\right)^T\mathbf{A}^{(k)}\right)$ separately.

To bound the first term, we note that by Cauchy-Schwarz inequality,

$$\|\left(\mathbf{A}^{(l)}\right)^T\mathbf{A}^{(k)}\|_F^2 = \text{trace}\left(\mathbf{A}^{(l)}\left(\mathbf{A}^{(l)}\right)^T\mathbf{A}^{(k)}\left(\mathbf{A}^{(k)}\right)^T\right) \le \|\Gamma^{(l)}\|_F\|\Gamma^{(k)}\|_F, \qquad \text{(S3.53)}$$

where we set $\Gamma^{(l)} = \mathbf{A}^{(l)}\left(\mathbf{A}^{(l)}\right)^T$. In addition, we have

$$\begin{aligned} & \|\Gamma^{(l)}\|_F^2 = \sum_{i=1}^{N_1}\|\Gamma^{(l),i}\|_F^2 \\ =\ & \sum_{i=1}^{N_1}(M_i(\gamma_0^l)^2 + 2(M_i-1)(\gamma_1^l)^2 + \ldots + 2(\gamma_{M_i-1}^l)^2) \\ \le\ & CN_1m_0\sum_{j=0}^{C_mm_0-1}(\gamma_j^l)^2 \le \begin{cases} CN_1m_0 & \text{if } \nu > 3/4 \\ CN_1m_0\log m_0 & \text{if } \nu = 3/4 \\ CN_1m_0^{4-4\nu} & \text{if } 1/2 < \nu < 3/4 \end{cases}, \qquad \text{(S3.54)} \end{aligned}$$

where the last inequality follows from Lemma 9 (ii).

To bound the second term, we note that

$$\lambda_{\max}\left(\left(\mathbf{A}^{(l)}\right)^T \mathbf{A}^{(k)}\right) \le \lambda_{\max}\left(\Gamma^{(l)}\right)^{1/2} \lambda_{\max}\left(\Gamma^{(k)}\right)^{1/2}. \tag{S3.55}$$

In addition, due to the block structure of $\Gamma^{(l)}$, we have

$$\lambda_{\max}\left(\Gamma^{(l)}\right) = \max_{i=1,\ldots,N_1}\left\{\lambda_{\max}\left(\Gamma^{(l),i}\right)\right\} \le 2\sum_{j=0}^{C_m m_0}\gamma_j^{(l)} \le \begin{cases} C & \text{if } \nu > 1 \\ C\log m_0 & \text{if } \nu = 1 \\ C m_0^{2-2\nu} & \text{if } 1/2 < \nu < 1 \end{cases}, \tag{S3.56}$$

where the last inequality is due to Lemma 9 (i).

Plugging equations (S3.53)-(S3.56) into equation (S3.52), we obtain that with probability at least $1 - O(p^{-(L+2)})$,

$$|T_1| \le \begin{cases} C\left(\sqrt{\frac{\log p}{N_k m_0}} + \frac{\log p}{N_k m_0}\right) & \text{if } \nu > 1 \\ C\left(\sqrt{\frac{\log p}{N_k m_0}} + \frac{\log p \log^2 m_0}{N_k m_0}\right) & \text{if } \nu = 1 \\ C\left(\sqrt{\frac{\log p}{N_k m_0}} + \frac{\log p}{N_k m_0^{2\nu-1}}\right) & \text{if } 3/4 < \nu < 1 \\ C\left(\sqrt{\frac{\log p \log m_0}{N_k m_0}} + \frac{\log p}{N_k m_0^{1/2}}\right) & \text{if } \nu = 3/4 \\ C\left(\sqrt{\frac{\log p}{N_k m_0^{4\nu-2}}} + \frac{\log p}{N_k m_0^{2\nu-1}}\right) & \text{if } 1/2 < \nu < 3/4 \end{cases}.$$

In the end, the result (ii) of the first part immediately follows from a union bound argument by plugging the bounds of $T_1$ and $T_2$ above into equation (S3.51). We point out that the upper bound of $T_1$ dominates that of $T_2$. Therefore, we complete the proof. □

**Proof of Lemma 7**

*Proof.* The proof of this lemma is essentially similar to that of Lemma 3. Recall that $\|\beta_k\|_1 \leq C_\beta$ for $k = 1, 2$. Therefore, by Hölder's inequality we have

$$\begin{aligned} & \left\|\hat{\Sigma}_k \beta_k - \hat{\mu}_k\right\|_\infty \\ \leq & \left\|\hat{\Sigma}_k - \Sigma_k\right\|_\infty \|\beta_k\|_1 + \|\mu_k - \hat{\mu}_k\|_\infty \\ \leq & \left\|\hat{\Sigma}_k - \Sigma_k\right\|_\infty C_\beta + \|\mu_k - \hat{\mu}_k\|_\infty . \end{aligned}$$

Consequently, the fact that $(\beta_1, \beta_2)$ is feasible with probability at least $1 - O(p^{-L})$ immediately follows from our choice of $\lambda_{2,N}$, the fact that $\log p \leq c_0 N$ and results (i)-(ii) in the second part of Lemma 6. It is worthwhile to point out that according to the fact $\log p \leq c_0 N$ and the bounds provided in Lemma 6, $\left\|\hat{\Sigma}_k \beta_k - \hat{\mu}_k\right\|_\infty$ is dominated by the term $\|\mu_k - \hat{\mu}_k\|_\infty$. □

**Proof of Lemma 8**

*Proof.* The proof of this lemma is similar to that of Lemma 5. We only highlight the main differences briefly below. The first inequality follows from the definitions of $\tilde{Z}_i$ and $Z_i$ directly. We show the second inequality holds below with probability at least $1 - O(p^{-(L+1)})$ for the fixed $i$. Without loss of generality, we assume $\mathcal{Y}_i = 1$ and $M_i = m_0 c_m$.

Following the lines in the proof of Lemma 5, we still can show that $\frac{1}{m_0 c_m} \left|\log\left(\frac{\hat{\pi}_1 \pi_2}{\hat{\pi}_2 \pi_1}\right)\right| \leq C_{z1} \max_{k=1,2} |\pi_k - \hat{\pi}_k|/m_0$ with some constant $C_{z1}$.

To deal with the term $|\bar{X}_i^T(\tilde{\beta} - \beta)|$, we note that with probability at least $1 - O(p^{-L-1})$

$$\begin{aligned} & |\bar{X}_i^T(\tilde{\beta} - \beta)| \leq \|\bar{X}_i\|_\infty \|\tilde{\beta} - \beta\|_1 \\ \leq & (\|\mu_1\|_\infty + U_\beta)\|\tilde{\beta} - \beta\|_1 \\ \leq & C(1 + U_\beta)\|\tilde{\beta} - \beta\|_1, \end{aligned} \quad \text{(S3.57)}$$

where the first inequity is due to Cauchy-Schwarz inequality, the second one follows from result (i) in the first part of Lemma 6 with $N_1 = 1$, and the last one is due to the fact that $\|\mu_1\| \leq C_\mu$.

Finally, we provide an upper bound for $\frac{1}{M_i}\left|\sum_{j=1}^{M_i} X_{ij}^T(\tilde{\nabla} - \nabla)X_{ij}/2\right|$. Set $U_{ij} := X_{ij} - \mu_1$. We still decompose it as we did in the proof of Lemma 5,

$$
\begin{aligned}
& \frac{1}{M_i}\left|\sum_{j=1}^{M_i} X_{ij}^T\left(\tilde{\nabla} - \nabla\right)X_{ij}/2\right| \\
\leq\ & \frac{1}{M_i}\left|\sum_{j=1}^{M_i} U_{ij}^T\left(\tilde{\nabla} - \nabla\right)U_{ij}/2\right| + \left|\mu_1^T\left(\tilde{\nabla} - \nabla\right)\mu_1/2\right| + \frac{1}{M_i}\left|\sum_{j=1}^{M_i} \mu_1^T\left(\tilde{\nabla} - \nabla\right)U_{ij}\right|.
\end{aligned}
$$

The second term still can be bounded as $|\mu_1^T(\tilde{\nabla}-\nabla)\mu_1/2| \leq C_\mu^2\|\tilde{\nabla}-\nabla\|_1/2$ by the assumption $\|\mu_1\| \leq C_\mu$. To bound the first term $(\sum_{j=1}^{M_i}\mu_1^T(\tilde{\nabla}-\nabla)U_{ij})/M_i$, we note that with probability at least $1 - O(p^{-L-1})$,

$$
\begin{aligned}
\frac{1}{M_i}\left|\sum_{j=1}^{M_i} \mu_1^T\left(\tilde{\nabla} - \nabla\right)U_{ij}\right| &\leq \|\frac{1}{M_i}\sum_{j=1}^{M_i} U_{ij}\|_\infty \|\mu_1^T\left(\tilde{\nabla} - \nabla\right)\|_1 \\
&\leq CU_\beta C_\mu \|\tilde{\nabla} - \nabla\|_1,
\end{aligned}
$$

where we used result (i) in the first part of Lemma 6 with $N_1 = 1$ during the last inequality above. To bound the third term, by Hölder's inequality, we have with probability at least

$1 - O(p^{-L-1})$,

$$\frac{1}{M_i}\left|\sum_{j=1}^{M_i} U_{ij}^T\left(\tilde{\nabla}-\nabla\right)U_{ij}/2\right| = \left|\mathrm{tr}(\left(\tilde{\nabla}-\nabla\right)\sum_{j=1}^{M_i} U_{ij}^T U_{ij}/M_i)/2\right|$$

$$\leq \frac{1}{2}\left\|\tilde{\nabla}-\nabla\right\|_1 \left\|\sum_{j=1}^{M_i} U_{ij}^T U_{ij}/M_i\right\|_\infty$$

$$\leq \begin{cases} C\left\|\tilde{\nabla}-\nabla\right\|_1\left(\sqrt{\frac{\log p}{m_0}}+\frac{\log p}{m_0}\right) & \text{if } \nu > 1 \\ C\left\|\tilde{\nabla}-\nabla\right\|_1\left(\sqrt{\frac{\log p}{m_0}}+\frac{\log p \log^2 m_0}{m_0}\right) & \text{if } \nu = 1 \\ C\left\|\tilde{\nabla}-\nabla\right\|_1\left(\sqrt{\frac{\log p}{m_0}}+\frac{\log p}{m_0^{2\nu-1}}\right) & \text{if } 3/4 < \nu < 1 \\ C\left\|\tilde{\nabla}-\nabla\right\|_1\left(\sqrt{\frac{\log p \log m_0}{m_0}}+\frac{\log p}{m_0^{1/2}}\right) & \text{if } \nu = 3/4 \\ C\left\|\tilde{\nabla}-\nabla\right\|_1\left(\sqrt{\frac{\log p}{m_0^{4\nu-2}}}+\frac{\log p}{m_0^{2\nu-1}}\right) & \text{if } 1/2 < \nu < 3/4 \end{cases},$$

where we have applied the bound of $|T_1|$ in the proof of Lemma 6 with $N_1 = 1$ in the last inequality above.

Combining the upper bounds of three terms above, we finally obtain that with probability $1 - O(p^{-L-1})$,

$$\frac{1}{M_i}\left|\sum_{j=1}^{M_i} X_{ij}^T\left(\tilde{\nabla}-\nabla\right)X_{ij}/2\right| \leq C(1+U_\nabla)\|\tilde{\nabla}-\nabla\|_1.$$

To complete our proof, we combine all bounds for $\frac{1}{m_0 c_m}\left|\log\left(\frac{\hat{\pi}_1\pi_2}{\hat{\pi}_2\pi_1}\right)\right|$, $|\bar{X}_i^T(\tilde{\beta}-\beta)|$ and $\frac{1}{M_i}|\sum_{j=1}^{M_i} X_{ij}^T(\tilde{\nabla}-\nabla)X_{ij}/2|$. □

# Bibliography

Bach, F. et al. (2010). Self-concordant analysis for logistic regression. *Electronic Journal of Statistics*, 4:384–414.

Beran, J. (2017). *Statistics for long-memory processes.* Routledge.

Chen, X., Xu, M., and Wu, W. B. (2016). Regularized estimation of linear functionals of precision matrices for high-dimensional time series. *IEEE Trans. Signal Processing*, 64(24):6459–6470.

Davidson, K. R. and Szarek, S. J. (2001). Local operator theory, random matrices and Banach spaces. *Handbook of the Geometry of Banach Spaces*, 1:317–366.

Dinov, I. D., Boscardin, J. W., Mega, M. S., Sowell, E. L., and Toga, A. W. (2005). A wavelet-based statistical analysis of fMRI data. *Neuroinformatics*, 3(4):319–342.

Johnstone, I. (2001). Thresholding for weighted $\chi^2$. *Statistica Sinica*, 11:691–704.

Laurent, B. and Massart, P. (2000). Adaptive estimation of a quadratic functional by model selection. *The Annals of Statistics*, 28(5):1302–1338.

Posekany, A., Felsenstein, K., and Sykacek, P. (2011). Biological assessment of robust noise models in microarray data analysis. *Bioinformatics*, 27(6):807–814.

Rudelson, M. and Vershynin, R. (2013). Hanson-Wright inequality and sub-gaussian concentration. *Electronic Communications in Probability*, 18(82):1–9.

Vershynin, R. (2012). Introduction to the non-asymptotic analysis of random matrices. *In Compressed Sensing, Theory and Applications*, pages 210–268.

Wu, W. B., Huang, Y., and Zheng, W. (2010). Covariances estimation for long-memory processes. *Advances in Applied Probability*, 42(1):137–157.

Zhao Ren

Department of Statistics, University of Pittsburgh, Pittsburgh, PA 15260, USA

E-mail:zren@pitt.edu

Sungkyu Jung

Department of Statistics, Seoul National University, Gwanak-gu, Seoul 08826, Korea

E-mail: sungkyu@snu.ac.kr

Xingye Qiao

Department of Mathematical Sciences, Binghamton University, State University of New York, Binghamton, NY, 13902 USA

E-mail: qiao@math.binghamton.edu
